# Supplementary material for: Bimetric interactions based on metric congruences
Source: arXiv:1906.11841 ancillary file (2019-06-27)
Supplement: Supplementary file 1 [file bim-cong-proofs-anc.pdf]

# Bimetric interactions based on congruences

Mikica Kocic, (L<sup>A</sup>T<sub>E</sub>X generated on 2019-06-02 13:44:28)

This file was generated by `bim-cong-proofs.nb`. The notebook `bim-cong-proofs.nb` contains the proofs of various identities that involve elementary symmetric polynomials. The identities were first derived by hand (incrementally, so the derivations could be tracked), then each step of the derivation was verified in *Mathematica*.

## Changelog

2015-04-11 Unconstrained bimetric potential based on metric contgurences  
2015-04-28 Identities involving symmetric polynomials  
2015-05-01 Varying the potential wrt  $p$ , obtained EoM and  $\Delta n = 0$   
2015-05-03 Vandermonde reparametrization  
2015-05-04 Solving for symmetrizing  $\Lambda$  (the final result)  
2017-12-02 Optimized the proof functions  
2017-12-22 Proof functions moved to a package (to be used with the geometric mean paper)  
2017-02-12 Refactoring Lorentz factor to  $\lambda$ , the shift of  $h$  to  $q$   
2019-05-12 Refactoring, put hats on all spatial restrictions  
2019-05-14 Split into: “definitions.nb”, “bim-cong-proofs.nb”, and “geom-mean-paper.nb”  
2019-05-16 LaTeX report generator

## Part 1

### Propositions involving $e_n$ and $Y_n$

The following claims hold for an arbitrary  $d$ -dimensional matrix  $X$ .

#### Partition of ESP

$$e_d(X)e_n(X^{-1}) = e_{d-n}(X) \quad (1)$$

**Recursive relation for  $Y_n(X) = \partial e_{n+1}(X) / \partial X^\top$**

$$Y_n(X) = \sum_{k=0}^n (-1)^{n+k} e_k(X) X^{n-k} \quad (2)$$

$$Y_0(X) = I \quad (3)$$

$$Y_{-1}(X) = 0 \quad (4)$$

$$Y_n(X) = e_n(X)I - XY_{n-1}(X) \quad (5)$$

## Damour's algebraic identity

$$\tilde{Y}_n(X) = \sum_{k=0}^{d-n} (-1)^{d-n+k} e_k(X^{-1}) X^{-(d-n-k)} \quad (6)$$

$$\tilde{Y}_0(X) = 0 \quad (7)$$

$$\tilde{Y}_{-1}(X) = 0 \quad (8)$$

$$\tilde{Y}_n(X) = Y_{d-n}(X^{-1}) \quad (9)$$

$$Y_n(X) + e_d(X) Y_{d-n}(X^{-1}) = e_n(X) I \quad (10)$$

$$Y_n(X) + \det(X) \tilde{Y}_n(X) = e_n(X) I \quad (11)$$

## Identities involving the projections $e_n(I + UW^\top)$

Here,  $U$  and  $W$  are  $d$ -dimensional column vectors. Matrices having the form  $I + UW^\top$  are part of the Lorentz transformations, the square roots and the projections.

$$ne_n(X) = \sum_{k=1}^n (-1)^{k-1} e_{n-k}(X) \operatorname{Tr}(X^k) \quad (12)$$

$$e_n(X + UW^\top) = \sum_{k=1}^n (-1)^{k-1} e_{n-k}(X) \operatorname{Tr}(X^{k-1} (\frac{1}{n} X + UW^\top)) \quad (13)$$

$$= e_n(X) + \sum_{k=1}^n (-1)^{k-1} e_{n-k}(X) W^\top X^{k-1} U \quad (14)$$

$$e_n(X(I + UW^\top)) = e_n(X) + \sum_{k=1}^n (-1)^{k-1} e_{n-k}(X) W^\top X^k U \quad (15)$$

$$= e_n(X) + W^\top X \sum_{k=0}^{n-1} (-1)^{n-1+k} e_k(X) X^{n-1-k} U \quad (16)$$

$$Y_n(X) = \sum_{k=0}^n (-1)^{n+k} e_k(X) X^{n-k} \quad (17)$$

$$e_n(X(I + UW^\top)) = e_n(X) + W^\top X Y_{n-1}(X) U \quad (18)$$

$$= e_n(X) + W^\top (e_n(X) I - Y_n(X)) U \quad (19)$$

$$= e_n(X) (1 + W^\top U) - W^\top Y_n(X) U \quad (20)$$

$$e_n(X + UW^\top) = e_n(X) + \sum_{k=1}^n (-1)^{k-1} e_{n-k}(X) W^\top X^{k-1} U \quad (21)$$

$$= e_n(X) + \sum_{k=0}^{n-1} (-1)^{n-1+k} e_k(X) W^\top X^{n-1-k} U \quad (22)$$

$$= e_n(X) + W^\top Y_{n-1}(X) U \quad (23)$$

$$= e_n(X) + W^\top (e_{n-1}(X) I - X Y_{n-2}(X)) U \quad (24)$$

$$= e_n(X) + e_{n-1}(X) W^\top U - W^\top X Y_{n-2}(X) U \quad (25)$$

### Cayley-Hamilton theorem and the related identities

The following claims hold for an arbitrary  $(d-1)$ -dimensional matrix  $D$ .

$$\sum_{k=0}^d (-1)^{d-k} e_{d-k}(D) D^k = 0 \quad (26)$$

$$\sum_{k=0}^{d-1} (-1)^{d-1-k} e_{d-1-k}(D) D^k = 0 \quad (27)$$

$$\sum_{k=1}^{d-n} (-1)^{k-1} e_{d-n-k}(D) D^k = \sum_{k=n+1}^d (-1)^{k-(n+1)} e_{d-k}(D) D^{k-n} \quad (28)$$

$$= \sum_{k=n+1}^d (-1)^{k-(n+1)} e_{d-k}(D) D^k D^{-n} \quad (29)$$

$$= \sum_{k=n}^{d-1} (-1)^{k-n} e_{d-1-k}(D) D^k D^{-n+1} \quad (30)$$

$$= - \sum_{k=0}^{n-1} (-1)^{k-n} e_{d-1-k}(D) D^k D^{-n+1} \quad (31)$$

$$= - \det(D) \sum_{k=0}^{n-1} (-1)^{k-n} e_k(D^{-1}) D^k D^{-n+1} \quad (32)$$

$$= - \det(D) \sum_{k=0}^{n-1} (-1)^{n-1-k-n} e_{n-1-k}(D^{-1}) D^{n-1-k} D^{-n+1} \quad (33)$$

$$= - \det(D) \sum_{k=1}^n (-1)^{n-k-n} e_{n-k}(D^{-1}) D^{n-k} D^{-n+1} \quad (34)$$

$$= \det(D) \sum_{k=1}^n (-1)^{k-1} e_{n-k}(D^{-1}) D^{-(k-1)} \quad (35)$$

### Lorentz transformation $\Lambda$

The following claims hold for an arbitrary  $(d-1)$ -dimensional vector  $v$  (not restricted to  $|v| < 1$ ).

$$\eta = \Lambda^\top \eta \Lambda \quad (36)$$

$$\Lambda = \begin{pmatrix} \lambda & p^\top \hat{\delta} \\ p & \hat{\Lambda} \end{pmatrix} \quad (37)$$

$$p = \lambda v \quad (38)$$

### The temporal part of $\Lambda$

$$\lambda^2 = 1 + p^\top \hat{\delta} p = (1 - v^\top \hat{\delta} v)^{-1} \quad (39)$$

The spatial part of  $\Lambda$

$$\hat{\Lambda} = \hat{I} + \frac{\lambda^2}{\lambda + 1} vv^\top \hat{\delta} \quad (40)$$

$$\hat{\Lambda}^2 = \hat{I} + pp^\top \hat{\delta} = \hat{I} + \lambda^2 vv^\top \hat{\delta} \quad (41)$$

$$\hat{\Lambda}^{-1} = \hat{I} - \frac{\lambda}{\lambda + 1} vv^\top \hat{\delta} = \hat{I} - \frac{1}{\lambda(\lambda + 1)} pp^\top \hat{\delta} \quad (42)$$

$$\hat{\Lambda}^{-2} = \hat{I} - vv^\top \hat{\delta} = \hat{I} - \lambda^{-2} pp^\top \hat{\delta} \quad (43)$$

$$\hat{\delta} \hat{\Lambda} = (\hat{\delta} \hat{\Lambda})^\top = \hat{\Lambda}^\top \hat{\delta} \quad (44)$$

The eigenvalues (all but one are 1)

$$\hat{\Lambda} v = \lambda v \quad (45)$$

$$\det(\hat{\Lambda}) = \lambda \quad (46)$$

## Part 2

Setup the metrics and verify relations between the variables

Metrics, vielbeins, and spatial metrics

$$g = E^\top \eta E \quad (47)$$

$$f = L^\top \eta L \quad (48)$$

$$\hat{g} = \text{spatial}(g) \quad (49)$$

$$\hat{f} = \text{spatial}(f) \quad (50)$$

Vielbeins

$$E = \begin{pmatrix} N & 0 \\ e\nu & e \end{pmatrix} \quad (51)$$

$$L = \begin{pmatrix} u^0 + u^\top q & u^\top \\ \hat{L}q & \hat{L} \end{pmatrix} = \begin{pmatrix} \lambda & \lambda v^\top \hat{\delta} \\ \lambda v & \hat{\Lambda} \end{pmatrix} \begin{pmatrix} M & 0 \\ m\mu & m \end{pmatrix} \quad (52)$$

General parametrization of the vielbein  $L$

$$\hat{L} = \hat{\Lambda} m \quad (53)$$

$$u^0 = \lambda^{-1} M \quad (54)$$

$$u = (v^\top \hat{\delta} \hat{\Lambda} m)^\top \quad (55)$$

$$q = M m^{-1} v + \mu \quad (56)$$

$$\hat{f} = -u u^\top + \hat{L}^\top \hat{\delta} \hat{L} \quad (57)$$

**The  $N + 1$  decomposition of the vielbein  $L$**

$$\textcolor{red}{M} = \lambda \textcolor{red}{u}^0 \quad (58)$$

$$\textcolor{red}{m} = \hat{\textcolor{green}{L}}^{-1} \hat{\textcolor{red}{L}} \quad (59)$$

$$\textcolor{red}{\mu} = \textcolor{red}{q} - \textcolor{red}{M} \textcolor{red}{m}^{-1} \textcolor{red}{v} \quad (60)$$

$$\textcolor{red}{v} = (\textcolor{violet}{u}^\top \hat{\textcolor{red}{L}}^{-1} \hat{\delta}^{-1})^\top \quad (61)$$

Check if the vielbein  $L$  is a proper one,

$$\textcolor{red}{v}^\top \hat{\delta} \textcolor{red}{v} < 1 \quad (62)$$

**At this point, we do not have a square root (!)**

$$\Delta \textcolor{violet}{n} = (\textcolor{blue}{N} \textcolor{blue}{e}^{-1} + \textcolor{red}{M} \textcolor{red}{m}^{-1}) \textcolor{red}{v} + \textcolor{red}{\mu} - \textcolor{red}{\nu} \quad (63)$$

$$\Delta \textcolor{violet}{n} \neq 0 \quad (64)$$

$$\hat{\delta} \hat{\textcolor{green}{L}} \textcolor{red}{m} \textcolor{blue}{e}^{-1} \neq (\hat{\delta} \hat{\textcolor{green}{L}} \textcolor{red}{m} \textcolor{blue}{e}^{-1})^\top \quad (65)$$

**Congruence  $\hat{B}$  (where  $\hat{B}$  is the spatial part of  $S$  that is pulled by  $e$ )**

$$\hat{B} = \textcolor{blue}{e}^{-1} \hat{\textcolor{green}{L}} \textcolor{red}{m} = \textcolor{blue}{e}^{-1} \hat{\textcolor{red}{L}} \quad (66)$$

$$\hat{B}^\top \hat{g} \hat{B} = \hat{\textcolor{red}{L}}^\top \hat{\delta} \hat{\textcolor{red}{L}} = \hat{\textcolor{red}{f}} + \textcolor{violet}{u} \textcolor{violet}{u}^\top \quad (67)$$

**Lorentz transformation in terms of  $f$**

$$\lambda^{-2} = x \quad (68)$$

$$Q = \textcolor{red}{m}^{-1} \hat{\textcolor{green}{L}} \hat{\textcolor{green}{L}} \textcolor{red}{m} = \hat{\textcolor{green}{I}} + \lambda^2 \widetilde{\textcolor{red}{n}} \widetilde{\textcolor{red}{n}}^\top \hat{\textcolor{red}{f}} \quad (69)$$

$$\hat{\textcolor{red}{f}} Q = Q^\top \hat{\textcolor{red}{f}} \quad (70)$$

$$\hat{B}^\top \hat{g} \hat{B} = \hat{\textcolor{red}{f}} Q = \hat{\textcolor{red}{f}} + \textcolor{violet}{u} \textcolor{violet}{u}^\top \quad (71)$$

**Relations between  $\hat{D}$  and  $\hat{B}$**

$$\hat{B} = \hat{D} Q \quad (72)$$

$$\hat{D}_g = Q^{-1} \hat{D}^{-1} \quad (73)$$

## The determinants of $S$ , $\hat{D}$ and $\hat{B}$

$$\det(S) = e_d(S) \quad (74)$$

$$= e_d(\hat{D}) + M(N\lambda)^{-1} e_{d-1}(\hat{B}) = M(N\lambda)^{-1} e_{d-1}(\hat{B}) \quad (75)$$

$$= M(N\lambda)^{-1} \det(\hat{B}) = M(N\lambda)^{-1} \det(\hat{D}Q) \quad (76)$$

$$\det(Q) = \lambda^2 \quad (77)$$

$$\det(S) = M\lambda N^{-1} \det(\hat{D}) \quad (78)$$

$$(\det(S))^{-1} = N(M\lambda)^{-1} \det(\hat{D}^{-1}) \quad (79)$$

## The decomposition of $e_n(S)$

The identities below are modified step-by-step (with minimal changes between two consecutive equations). The derivations are done in several branches. The last branch contains the expression for  $Ne_n(S)$  that is varied to get EoM.

The main expressions equal to  $\boxed{Ne_n(S)}$

$$\text{Established } Ne_n(S): \quad (80)$$

$$Ne_n(S) = Ne_n(\hat{B}) + u^0 e_{n-1}(\hat{B}) + \sum_{k=1}^n (-1)^{k-1} e_{n-k}(\hat{B}) u^\top \hat{B}^{k-1} (q - \nu) \quad (81)$$

$$= Ne_n(\hat{D}) + u^0 e_{n-1}(\hat{B}) + \sum_{k=1}^n (-1)^{k-1} e_{n-k}(\hat{B}) u^\top \hat{B}^{k-1} \Delta n \quad (82)$$

$$= Ne_n(\hat{D}) + u^0 e_{n-1}(\hat{B}) + e_n(\hat{B} + \Delta n u^\top) - e_n(\hat{B}) \quad (83)$$

$$= Ne_n(\hat{B}) + \lambda^{-1} M e_{n-1}(\hat{B}) + \lambda \sum_{k=1}^n (-1)^{k-1} e_{n-k}(\hat{B}) \tilde{n}^\top \hat{f} \hat{B}^{k-1} (q - \nu) \quad (84)$$

$$= Ne_n(\hat{D}) + \lambda^{-1} M e_{n-1}(\hat{B}) + \lambda \sum_{k=1}^n (-1)^{k-1} e_{n-k}(\hat{B}) \tilde{n}^\top \hat{f} \hat{B}^{k-1} \Delta n \quad (85)$$

$$\sqrt{-g} e_n(S) = N \det(e) e_n(\hat{D}) + M \det(m) e_{d-n}(\hat{D}_g) + \det(e) \sum_{k=1}^n (-1)^{k-1} e_{n-k}(\hat{B}) \lambda \tilde{n}^\top \hat{f} \hat{B}^{k-1} \Delta n \quad (86)$$

**Strategy:** We should rewrite  $Ne_n(S)$  to obtain the equations that contain an isolated  $p$  together with the elementary symmetric polynomials which are of the form  $Ne_n(me^{-1})$  or  $Ne_n(em^{-1})$ .

$\boxed{Ne_n(S)}$  **Derivation track 1**

$$\begin{aligned} Ne_n(S) &= Ne_n(e^{-1} \hat{\Lambda} m) + \lambda^{-1} M e_{n-1}(e^{-1} \hat{\Lambda} m) - e_n(\hat{B}) \\ &\quad + e_n(e^{-1} \hat{\Lambda} m + (M m^{-1} v + \mu - \nu) v^\top \hat{\delta} \hat{\Lambda} m) \\ &= Ne_n(e^{-1} \hat{\Lambda} m) + \lambda^{-1} M e_{n-1}(e^{-1} \hat{\Lambda} m) - e_n(e^{-1} \hat{\Lambda} m - M m^{-1} v v^\top \hat{\delta} \hat{\Lambda} m) \end{aligned} \quad (87)$$

$$+ e_n(e^{-1}\hat{\Lambda}m + (\mu - \nu)v^\top \hat{\delta}\hat{\Lambda}m) \quad (88)$$

$$= Ne_n(me^{-1}\hat{\Lambda}) + \lambda^{-1}Me_{n-1}(me^{-1}\hat{\Lambda}) - e_n(me^{-1}\hat{\Lambda} - \lambda Mvv^\top \hat{\delta}) \\ + e_n(me^{-1}\hat{\Lambda} + \lambda m(\mu - \nu)v^\top \hat{\delta}) \quad (89)$$

$$= Ne_n(me^{-1}\hat{\Lambda}) + \lambda^{-1}M(e_{n-1}(me^{-1}\hat{\Lambda}) \\ - \lambda^2 \sum_{k=0}^{n-1} (-1)^{k-1} e_{n-1-k}(me^{-1}\hat{\Lambda})v^\top \hat{\delta}(me^{-1}\hat{\Lambda})^k v) \\ + e_n(me^{-1}\hat{\Lambda} + \lambda m(\mu - \nu)v^\top \hat{\delta}) - e_n(me^{-1}\hat{\Lambda}) \quad (90)$$

$$= Ne_n(me^{-1}\hat{\Lambda}) \\ + \lambda^{-1}M(e_{n-1}(me^{-1}\hat{\Lambda}) \\ - \lambda^2 \sum_{k=1}^{n-1} (-1)^{k-1} e_{n-1-k}(me^{-1}\hat{\Lambda})v^\top \hat{\delta}(me^{-1}\hat{\Lambda})^k v + \lambda^2 e_{n-1}(me^{-1}\hat{\Lambda})v^\top \hat{\delta}v) \\ + e_n(me^{-1}\hat{\Lambda} + \lambda m(\mu - \nu)v^\top \hat{\delta}) - e_n(me^{-1}\hat{\Lambda}) \quad (91)$$

$$= Ne_n(me^{-1}\hat{\Lambda}) + \lambda^{-1}M[e_{n-1}(me^{-1}\hat{\Lambda}(\hat{I} - \lambda^2 vv^\top \hat{\delta})) + e_{n-1}(me^{-1}\hat{\Lambda})\lambda^2 v^\top \hat{\delta}v] \\ + e_n(me^{-1}\hat{\Lambda} + \lambda m(\mu - \nu)v^\top \hat{\delta}) - e_n(me^{-1}\hat{\Lambda}) \quad (92)$$

$$= Ne_n(me^{-1}\hat{\Lambda}) + \lambda^{-1}M[e_{n-1}(me^{-1}\hat{\Lambda}(\hat{I} - pp^\top \hat{\delta})) + e_{n-1}(me^{-1}\hat{\Lambda})p^\top \hat{\delta}p] \\ + e_n(me^{-1}\hat{\Lambda} + m(\mu - \nu)p^\top \hat{\delta}) - e_n(me^{-1}\hat{\Lambda}) \quad (93)$$

### $Ne_n(S)$ Derivation track 2

$$= Ne_n(\hat{D}) + \lambda Me_{n-1}(\hat{D}) - \lambda M \sum_{k=1}^n (-1)^{k-1} e_{n-k}(\hat{D})\tilde{n}^\top \hat{f} \hat{D}^{k-1} \tilde{n} \\ + \lambda \sum_{k=1}^n (-1)^{k-1} e_{n-k}(\hat{B})\tilde{n}^\top \hat{f} \hat{B}^{k-1} \Delta n \quad (94)$$

$$= Ne_n(\hat{B}) + \lambda^{-1}Me_{n-1}(\hat{B}) + e_n(\hat{B} + \lambda(q - \nu)\tilde{n}^\top \hat{f}) - e_n(\hat{B}) \quad (95)$$

$$= Ne_n(\hat{B}) + \lambda^{-1}Me_{n-1}(\hat{B}) + Ne_n(\hat{B} + N^{-1}\lambda(q - \nu)\tilde{n}^\top \hat{f}) - Ne_n(\hat{B}) \quad (96)$$

$$= \lambda^{-1}Me_{n-1}(\hat{B}) + Ne_n(\hat{B} + N^{-1}\lambda(q - \nu)\tilde{n}^\top \hat{f}) \quad (97)$$

$$= \lambda^{-1}Me_{n-1}(\hat{B}) + Ne_n(\hat{B} + N^{-1}\lambda(q - \nu)\tilde{n}^\top \hat{f}) \quad (98)$$

$$= Ne_n(\hat{B}) + \lambda^{-1}Me_{n-1}(\hat{B}) + \lambda e_n(\hat{B} + (\mu - \nu)\tilde{n}^\top \hat{f}) - \lambda e_n(\hat{B}) \\ + \lambda^{-1}Me_n(\hat{B} + \lambda^2 m^{-1}v\tilde{n}^\top \hat{f}) - \lambda^{-1}Me_n(\hat{B}) \quad (99)$$

$$= Ne_n(\hat{B}) + \lambda^{-1}Me_{n-1}(\hat{B}) + e_n(\hat{B} + \lambda(\mu - \nu)\tilde{n}^\top \hat{f}) - e_n(\hat{B} - \lambda Mm^{-1}v\tilde{n}^\top \hat{f}) \quad (100)$$

### $N \det(e) e_n(S)$ Derivation track 3

$$\sqrt{-g}e_n(S) = N \det(e) e_n(S) \quad (101)$$

$$= M \det(m) e_{d-n}(S^{-1}) \quad (102)$$

$$= N \det(e) e_n(e^{-1}\hat{\Lambda}^{-1}m) + M \det(m) e_{d-n}(m^{-1}\hat{\Lambda}^{-1}e) - \det(e) e_n(e^{-1}\hat{\Lambda}m) \\ + \det(e) e_n(e^{-1}\hat{\Lambda}m + (Ne^{-1}v + Mm^{-1}v + \mu - \nu)v^\top \hat{\delta}\hat{\Lambda}m) \quad (103)$$

$$= M \det(m) e_{d-n}(m^{-1}\hat{\Lambda}^{-1}e) + N \det(e) e_n(e^{-1}\hat{\Lambda}^{-1}m) - \det(m) e_{d-n}(m^{-1}\hat{\Lambda}e) \\ + \det(m) e_{d-n}(m^{-1}\hat{\Lambda}e + (Ne^{-1}v + Mm^{-1}v + \mu - \nu)v^\top \hat{\delta}\hat{\Lambda}e) \quad (104)$$

$$\begin{aligned} \det(e) & \left[ e_n(e^{-1}\hat{\Lambda}m + (Ne^{-1}v + Mm^{-1}v + \mu - \nu)v^\top \hat{\delta}\hat{\Lambda}m) - e_n(e^{-1}\hat{\Lambda}m) \right] \\ & = \det(m) \left[ e_{d-n}(m^{-1}\hat{\Lambda}e + (Ne^{-1}v + Mm^{-1}v + \mu - \nu)v^\top \hat{\delta}\hat{\Lambda}e) - e_{d-n}(m^{-1}\hat{\Lambda}e) \right] \end{aligned} \quad (105)$$

$$\begin{aligned} \sqrt{-g}e_n(S) & = N \det(e) e_n(e^{-1}\hat{\Lambda}^{-1}m) + M \det(m) e_{d-n}(m^{-1}\hat{\Lambda}^{-1}e) \\ & \quad + \det(e) \left[ e_n(e^{-1}\hat{\Lambda}m + (Ne^{-1}v + Mm^{-1}v)v^\top \hat{\delta}\hat{\Lambda}m) - e_n(e^{-1}\hat{\Lambda}m - (\mu - \nu)v^\top \hat{\delta}\hat{\Lambda}m) \right] \end{aligned} \quad (106)$$

$$\begin{aligned} & = N \det(e) e_n(e^{-1}\hat{\Lambda}^{-1}m) + M \det(m) e_{d-n}(m^{-1}\hat{\Lambda}^{-1}e) \\ & \quad + \det(m) \left[ e_{d-n}(m^{-1}\hat{\Lambda}e + (Ne^{-1}v + Mm^{-1}v)v^\top \hat{\delta}\hat{\Lambda}e) - e_{d-n}(m^{-1}\hat{\Lambda}e - (\mu - \nu)v^\top \hat{\delta}\hat{\Lambda}e) \right] \end{aligned} \quad (107)$$

$$\begin{aligned} Ne_n(S) & = Ne_n(e^{-1}\hat{\Lambda}^{-1}m) + \lambda^{-1}Me_{n-1}(e^{-1}\hat{\Lambda}m) \\ & \quad + e_n(e^{-1}\hat{\Lambda}m + (Ne^{-1}v + Mm^{-1}v)v^\top \hat{\delta}\hat{\Lambda}m) - e_n(e^{-1}\hat{\Lambda}m - (\mu - \nu)v^\top \hat{\delta}\hat{\Lambda}m) \end{aligned} \quad (108)$$

$$\begin{aligned} & = Ne_n(e^{-1}\hat{\Lambda}m) + \lambda^{-1}Me_{n-1}(e^{-1}\hat{\Lambda}m) - e_n(e^{-1}\hat{\Lambda}m - Mm^{-1}vv^\top \hat{\delta}\hat{\Lambda}m) \\ & \quad + e_n(e^{-1}\hat{\Lambda}m + (\mu - \nu)v^\top \hat{\delta}\hat{\Lambda}m) \end{aligned} \quad (109)$$

$N \det(e) e_n(S)$  **Derivation track 4**

$$\begin{aligned} \sqrt{-g}e_n(S) & = N \det(e) e_n(e^{-1}\hat{\Lambda}^{-1}m + e^{-1}vv^\top \hat{\delta}\hat{\Lambda}m) + M \det(m) e_{d-n}(m^{-1}\hat{\Lambda}^{-1}e + m^{-1}vv^\top \hat{\delta}\hat{\Lambda}e) \\ & \quad + \det(e) e_n(e^{-1}\hat{\Lambda}m + (\mu - \nu)v^\top \hat{\delta}\hat{\Lambda}m) - \det(e) e_n(e^{-1}\hat{\Lambda}m) \end{aligned} \quad (110)$$

$$\begin{aligned} & = N \det(e) e_n(e^{-1}\hat{\Lambda}^{-1}m + e^{-1}vv^\top \hat{\delta}\hat{\Lambda}m) + M \det(m) e_{d-n}(m^{-1}\hat{\Lambda}^{-1}e + m^{-1}vv^\top \hat{\delta}\hat{\Lambda}e) \\ & \quad + \det(m) e_{d-n}(m^{-1}\hat{\Lambda}e + (\mu - \nu)v^\top \hat{\delta}\hat{\Lambda}e) - \det(m) e_{d-n}(m^{-1}\hat{\Lambda}e) \end{aligned} \quad (111)$$

$$\begin{aligned} & = N \det(e) e_n(e^{-1}\hat{\Lambda}^{-1}m + e^{-1}vv^\top \hat{\delta}\hat{\Lambda}m) + M \det(m) e_{d-n}(m^{-1}\hat{\Lambda}^{-1}e + m^{-1}vv^\top \hat{\delta}\hat{\Lambda}e) \\ & \quad + \det(e) e_n(e^{-1}\hat{\Lambda}m + (\mu - \nu)v^\top \hat{\delta}\hat{\Lambda}m) - \det(e) e_n(e^{-1}\hat{\Lambda}m) \end{aligned} \quad (112)$$

$$\begin{aligned} & e_n(e^{-1}\hat{\Lambda}m + (\mu - \nu)v^\top \hat{\delta}\hat{\Lambda}m) \\ & = e_n(e^{-1}\hat{\Lambda}m) + e_n(e^{-1}\hat{\Lambda}m + \mu v^\top \hat{\delta}\hat{\Lambda}m) - e_n(e^{-1}\hat{\Lambda}m + \nu v^\top \hat{\delta}\hat{\Lambda}m) \end{aligned} \quad (113)$$

$$\begin{aligned} \sqrt{-g}e_n(S) & = N \det(e) e_n(e^{-1}\hat{\Lambda}^{-1}m + e^{-1}vv^\top \hat{\delta}\hat{\Lambda}m) - \det(e) e_n(e^{-1}\hat{\Lambda}m + \nu v^\top \hat{\delta}\hat{\Lambda}m) \\ & \quad + M \det(m) e_{d-n}(m^{-1}\hat{\Lambda}^{-1}e + m^{-1}vv^\top \hat{\delta}\hat{\Lambda}e) + \det(e) e_n(e^{-1}\hat{\Lambda}m + \mu v^\top \hat{\delta}\hat{\Lambda}m) \end{aligned} \quad (114)$$

$N \det(e) e_n(S)$  **Derivation track 5**

$$\begin{aligned} & = N \det(e) e_n(e^{-1}\hat{\Lambda}^{-1}m + e^{-1}vv^\top \hat{\delta}\hat{\Lambda}m) - \det(e) e_n(e^{-1}\hat{\Lambda}m + \nu v^\top \hat{\delta}\hat{\Lambda}m) \\ & \quad + M \det(m) e_{d-n}(m^{-1}\hat{\Lambda}^{-1}e + m^{-1}vv^\top \hat{\delta}\hat{\Lambda}e) + \det(m) e_{d-n}(m^{-1}\hat{\Lambda}e + \mu v^\top \hat{\delta}\hat{\Lambda}e) \\ & \quad + \det(e) e_n(e^{-1}\hat{\Lambda}m) - \det(m) e_{d-n}(m^{-1}\hat{\Lambda}e) \end{aligned} \quad (115)$$

$$\begin{aligned} & = N \det(e) e_n(e^{-1}\hat{\Lambda}m) - \det(e) e_n(e^{-1}\hat{\Lambda}m + \nu v^\top \hat{\delta}\hat{\Lambda}m) + \det(e) e_n(e^{-1}\hat{\Lambda}m) \\ & \quad + M \det(m) e_{d-n}(m^{-1}\hat{\Lambda}e) + \det(m) e_{d-n}(m^{-1}\hat{\Lambda}e + \mu v^\top \hat{\delta}\hat{\Lambda}e) - \det(m) e_{d-n}(m^{-1}\hat{\Lambda}e) \end{aligned} \quad (116)$$

$$\begin{aligned} & = \det(e) (Ne_n(e^{-1}\hat{\Lambda}m) - e_n(e^{-1}\hat{\Lambda}m + \nu v^\top \hat{\delta}\hat{\Lambda}m) + e_n(e^{-1}\hat{\Lambda}m)) \\ & \quad + \det(m) (Me_{d-n}(m^{-1}\hat{\Lambda}e) + e_{d-n}(m^{-1}\hat{\Lambda}e + \mu v^\top \hat{\delta}\hat{\Lambda}e) - e_{d-n}(m^{-1}\hat{\Lambda}e)) \end{aligned} \quad (117)$$

$$= \det(e) \left[ Ne_n(m e^{-1}\hat{\Lambda}) - e_n(m e^{-1}(\hat{I} + \frac{1}{\lambda+1}pp^\top \hat{\delta} + e\nu p^\top \hat{\delta})) + e_n(m e^{-1}\hat{\Lambda}) \right]$$



$$+ \det(m) (Me_{d-n}(m^{-1}\hat{\Lambda}e) + e_{d-n}(m^{-1}\hat{\Lambda}e + \mu p^\top \hat{\delta}e) - e_{d-n}(m^{-1}\hat{\Lambda}e)) \quad (118)$$

The following is close to what we want (to be varied wrt  $p$ ).

$$\begin{aligned} &= \det(e) (Ne_n(me^{-1}) + \sum_{k=1}^n (-1)^{k-1} e_{n-k}(me^{-1}) p^\top \hat{\delta}(me^{-1})^k e (\frac{1}{\lambda+1} Ne^{-1}p - \nu)) \\ &\quad + \det(m) (Me_{d-n}(m^{-1}\hat{\Lambda}e) + e_{d-n}(m^{-1}\hat{\Lambda}e + \mu p^\top \hat{\delta}e) - e_{d-n}(m^{-1}\hat{\Lambda}e)) \end{aligned} \quad (119)$$

### $N \det(e) e_n(S)$ Derivation track 6

Here we get the elementary symmetric polynomials of the form  $Ne_n(me^{-1})$  or  $Ne_n(em^{-1})$ .

$$\begin{aligned} &= \det(e) (Ne_n(me^{-1}) \\ &\quad + \sum_{k=1}^n (-1)^{k-1} e_{n-k}(me^{-1}) p^\top \hat{\delta}(me^{-1})^k e (\frac{1}{\lambda+1} Ne^{-1}p - \nu)) \\ &\quad + \det(m) (Me_{d-n}(em^{-1}) \\ &\quad + \sum_{k=1}^{d-n} (-1)^{k-1} e_{d-n-k}(em^{-1}) p^\top \hat{\delta}(em^{-1})^k m (\frac{1}{\lambda+1} Mm^{-1}p + \mu)) \end{aligned} \quad (120)$$

$$\begin{aligned} &= N \det(e) (e_n(me^{-1}) \\ &\quad + \sum_{k=1}^n (-1)^{k-1} e_{n-k}(me^{-1}) p^\top \hat{\delta}(me^{-1})^k e (\frac{1}{\lambda+1} e^{-1}p - N^{-1}\nu)) \\ &\quad + M \det(m) (e_{d-n}(em^{-1}) \\ &\quad + \sum_{k=1}^{d-n} (-1)^{k-1} e_{d-n-k}(em^{-1}) p^\top \hat{\delta}(em^{-1})^k m (\frac{1}{\lambda+1} m^{-1}p + M^{-1}\mu)) \end{aligned} \quad (121)$$

$$\begin{aligned} &= N \det(e) e_n \left[ me^{-1} \left( \hat{I} + (\frac{1}{\lambda+1} p - N^{-1}e\nu) p^\top \hat{\delta} \right) \right] \\ &\quad + M \det(m) e_{d-n} \left[ em^{-1} \left( \hat{I} + (\frac{1}{\lambda+1} p + M^{-1}m\mu) p^\top \hat{\delta} \right) \right] \end{aligned} \quad (122)$$

$$\begin{aligned} &= N \det(e) e_n (me^{-1}(\hat{\Lambda} - N^{-1}e\nu p^\top \hat{\delta})) \\ &\quad + M \det(m) e_{d-n} (em^{-1}(\hat{\Lambda} + M^{-1}m\mu p^\top \hat{\delta})) \end{aligned} \quad (123)$$

$$\begin{aligned} &= N \det(e) e_n (me^{-1}\hat{\Lambda} - N^{-1}m\nu p^\top \hat{\delta}) \\ &\quad + M \det(m) e_{d-n} (em^{-1}\hat{\Lambda} + M^{-1}\mu p^\top \hat{\delta}) \end{aligned} \quad (124)$$

$$\begin{aligned} &= N \det(e) e_n (e^{-1}\hat{\Lambda}m - N^{-1}\nu v^\top \hat{\delta}\hat{\Lambda}m) \\ &\quad + M \det(m) e_{d-n} (m^{-1}\hat{\Lambda}e + M^{-1}\mu v^\top \hat{\delta}\hat{\Lambda}e) \end{aligned} \quad (125)$$

$$\begin{aligned} &= N \det(e) e_n ((e^{-1} - N^{-1}\nu v^\top \hat{\delta})\hat{\Lambda}m) \\ &\quad + M \det(m) e_{d-n} ((m^{-1} + M^{-1}\mu v^\top \hat{\delta})\hat{\Lambda}e) \end{aligned} \quad (126)$$

$$\begin{aligned} &= N \det(e) e_n \left[ (e^{-1} + N^{-1}(\frac{\lambda}{\lambda+1} Ne^{-1}v - \nu) v^\top \hat{\delta}\hat{\Lambda})m \right] \\ &\quad + M \det(m) e_{d-n} \left[ (m^{-1} + M^{-1}(\frac{\lambda}{\lambda+1} Mm^{-1}v + \mu) v^\top \hat{\delta}\hat{\Lambda})e \right] \end{aligned} \quad (127)$$

### $Ne_n(S)$ Derivation track 7 (used to get EoM)

Now the equations contain  $p$ 's outside the elementary symmetric polynomials (the parts which depend on  $p$  are highlighted in yellow). These equations are nice to be varied w.r.t.  $p$ .

$$= N \det(e) (e_n(me^{-1}))$$

$$\begin{aligned}
& + \sum_{k=1}^n (-1)^{k-1} e_{n-k}(\textcolor{red}{m}e^{-1}) p^\top \hat{\delta}(\textcolor{red}{m}e^{-1})^k e\left(\frac{1}{\lambda+1} e^{-1} p - N^{-1} \nu\right) \\
& + \textcolor{red}{M} \det(\textcolor{red}{m}) (e_{d-n}(\textcolor{red}{m}e^{-1}) \\
& + \sum_{k=1}^{d-n} (-1)^{k-1} e_{d-n-k}(\textcolor{red}{m}e^{-1}) p^\top \hat{\delta}(\textcolor{red}{m}e^{-1})^k \textcolor{red}{m} \left(\frac{1}{\lambda+1} \textcolor{red}{m}^{-1} p + \textcolor{red}{M}^{-1} \mu\right) \tag{128}
\end{aligned}$$

$$\begin{aligned}
& = N \det(e) e_n(\textcolor{red}{m}e^{-1}) \\
& + \det(e) \sum_{k=1}^n (-1)^{k-1} e_{n-k}(\textcolor{red}{m}e^{-1}) p^\top \hat{\delta}(\textcolor{red}{m}e^{-1})^k e\left(\frac{1}{\lambda+1} N e^{-1} p - \nu\right) \\
& + \textcolor{red}{M} \det(\textcolor{red}{m}) e_{d-n}(\textcolor{red}{m}e^{-1}) \\
& + \det(\textcolor{red}{m}) \sum_{k=1}^{d-n} (-1)^{k-1} e_{d-n-k}(\textcolor{red}{m}e^{-1}) p^\top \hat{\delta}(\textcolor{red}{m}e^{-1})^k \textcolor{red}{m} \left(\frac{1}{\lambda+1} \textcolor{red}{M} \textcolor{red}{m}^{-1} p + \mu\right) \tag{129}
\end{aligned}$$

$$\begin{aligned}
& = N \det(e) e_n(\textcolor{red}{m}e^{-1}) \\
& + \det(e) \sum_{k=1}^n (-1)^{k-1} e_{n-k}(\textcolor{red}{m}e^{-1}) p^\top \hat{\delta}(\textcolor{red}{m}e^{-1})^k e\left(\frac{1}{\lambda+1} N e^{-1} p - \nu\right) \\
& + \textcolor{red}{M} \det(e) e_{n-1}(\textcolor{red}{m}e^{-1}) \\
& + \det(e) \sum_{k=1}^n (-1)^{k-1} e_{n-k}(\textcolor{red}{m}e^{-1}) p^\top \hat{\delta}(\textcolor{red}{m}e^{-1})^k e\left(\frac{1}{\lambda+1} \textcolor{red}{M} \textcolor{red}{m}^{-1} p + \mu\right) \tag{130}
\end{aligned}$$

$$\begin{aligned}
& = N \det(e) e_n(\textcolor{red}{m}e^{-1}) \\
& + \det(e) \sum_{k=1}^n (-1)^{k-1} e_{n-k}(\textcolor{red}{m}e^{-1}) p^\top \hat{\delta}(\textcolor{red}{m}e^{-1})^k e\left(\frac{1}{\lambda+1} N e^{-1} p - \nu\right) \\
& + \textcolor{red}{M} \det(\textcolor{red}{m}) e_{d-n}(\textcolor{red}{m}e^{-1}) \\
& + \det(e) \sum_{k=1}^n (-1)^{k-1} e_{n-k}(\textcolor{red}{m}e^{-1}) p^\top \hat{\delta}(\textcolor{red}{m}e^{-1})^k e\left(\frac{1}{\lambda+1} \textcolor{red}{M} \textcolor{red}{m}^{-1} p + \mu\right) \tag{131}
\end{aligned}$$

Finally, we have  $\boxed{N e_n(S)}$  which is suitable to be varied

$$\begin{aligned}
N e_n(S) & = N e_n(\textcolor{red}{m}e^{-1}) + \textcolor{red}{M} e_{n-1}(\textcolor{red}{m}e^{-1}) \\
& + \sum_{k=1}^n (-1)^{k-1} e_{n-k}(\textcolor{red}{m}e^{-1}) p^\top \hat{\delta}(\textcolor{red}{m}e^{-1})^k e\left(\frac{1}{\lambda+1} N e^{-1} p + \frac{1}{\lambda+1} \textcolor{red}{M} \textcolor{red}{m}^{-1} p + \mu - \nu\right) \tag{132}
\end{aligned}$$

$$\begin{aligned}
& = N e_n(\textcolor{red}{m}e^{-1}) + \textcolor{red}{M} e_{n-1}(\textcolor{red}{m}e^{-1}) \\
& + \sum_{k=1}^n (-1)^{k-1} e_{n-k}(\textcolor{red}{m}e^{-1}) p^\top \hat{\delta}(\textcolor{red}{m}e^{-1})^{k-1} \textcolor{red}{m} \left((N e^{-1} + \textcolor{red}{M} \textcolor{red}{m}^{-1}) \frac{1}{\lambda+1} p + \mu - \nu\right) \tag{133}
\end{aligned}$$

The equations of motion will be obtained from the following:

$$\begin{aligned}
& = N e_n(\textcolor{red}{m}e^{-1}) + \textcolor{red}{M} e_{n-1}(\textcolor{red}{m}e^{-1}) \\
& + \sum_{k=1}^n (-1)^{k-1} e_{n-k}(\textcolor{red}{m}e^{-1}) p^\top \hat{\delta}(\textcolor{red}{m}e^{-1})^{k-1} \textcolor{red}{m} \left((N e^{-1} + \textcolor{red}{M} \textcolor{red}{m}^{-1}) \frac{1}{\lambda+1} p + \mu - \nu\right) \tag{134}
\end{aligned}$$

# Part 3

## Equations of Motion for $p$

The starting point is  $Ne_n(S)$

$$\text{Established } Ne_n(S): \quad (135)$$

$$\begin{aligned} Ne_n(S) &= Ne_n(me^{-1}) + Me_{n-1}(me^{-1}) \\ &\quad + \sum_{k=1}^n (-1)^{k-1} e_{n-k}(me^{-1}) p^\top \hat{\delta} (me^{-1})^{k-1} m ((Ne^{-1} + Mm^{-1}) \frac{1}{\lambda+1} p + \mu - \nu) \end{aligned} \quad (136)$$

$$\begin{aligned} &= Ne_n(me^{-1}) + Me_{n-1}(me^{-1}) \\ &\quad + p^\top \hat{\delta} Y_{n-1}(me^{-1}) m ((Ne^{-1} + Mm^{-1}) \frac{1}{\lambda+1} p + \mu - \nu) \end{aligned} \quad (137)$$

$$\begin{aligned} &= Ne_n(me^{-1}) + Me_{n-1}(me^{-1}) \\ &\quad + v^\top \hat{\Lambda}^\top \hat{\delta} Y_{n-1}(me^{-1}) m \left( \frac{\lambda}{\lambda+1} (Ne^{-1} + Mm^{-1}) v + \mu - \nu \right) \end{aligned} \quad (138)$$

The variation of  $Ne_n(S)$  with respect to  $p = \lambda v$

The variation  $\partial \mathcal{V} / \partial p$  is established using the following two identities:

$$\partial (p^\top \cdot \diamond) / \partial p = \diamond^\top,$$

$$\partial \left( \diamond \cdot \frac{p}{\lambda+1} \right) / \partial p = \frac{1}{\lambda+1} \diamond \cdot \hat{\Lambda}^{-1} \quad \text{where} \quad \hat{\Lambda}^{-1} = \hat{I} - \frac{1}{\lambda(\lambda+1)} p p^\top \hat{\delta},$$

where  $\diamond$  and  $\blacklozenge$  are assumed not to depend on  $p$ .

$$\text{Established } (\delta \mathcal{V}): \quad (139)$$

$$\begin{aligned} \delta \mathcal{V}^\top &= \hat{\delta} Y_{n-1}(me^{-1}) m \left( \frac{\lambda}{\lambda+1} (Ne^{-1} + Mm^{-1}) v + \mu - \nu \right) \\ &\quad + \frac{1}{\lambda+1} (v^\top \hat{\Lambda}^\top \hat{\delta} Y_{n-1}(me^{-1}) m (Ne^{-1} + Mm^{-1}) \hat{\Lambda}^{-1})^\top \end{aligned} \quad (140)$$

$$\begin{aligned} &= \hat{\delta} Y_{n-1}(me^{-1}) m ((Ne^{-1} + Mm^{-1}) v + \mu - \nu) \\ &\quad + \frac{1}{\lambda+1} (\hat{\Lambda}^\top \hat{\delta} Y_{n-1}(me^{-1}) m (Ne^{-1} + Mm^{-1}) \hat{\Lambda}^{-1})^\top v \\ &\quad - \frac{1}{\lambda+1} \hat{\delta} Y_{n-1}(me^{-1}) m (Ne^{-1} + Mm^{-1}) v \end{aligned} \quad (141)$$

If  $\hat{\delta} \hat{\Lambda} m e^{-1}$  is symmetric, then the following holds:

$$\hat{\delta} \hat{\Lambda} m e^{-1} = (\hat{\delta} \hat{\Lambda} m e^{-1})^\top \quad (142)$$

$$\hat{g}^{-1} \hat{f} = e^{-1} \hat{\Lambda} m e^{-1} \hat{\Lambda}^{-1} m \quad (143)$$

$$\hat{\delta} \hat{\Lambda} (m e^{-1})^n = (\hat{\delta} \hat{\Lambda} (m e^{-1})^n)^\top \quad (144)$$

This means that  $\hat{\delta} \hat{\Lambda} f(m e^{-1})$  is symmetric for any analytic function  $f$ .

$$\hat{\delta} \hat{\Lambda} \log(m e^{-1}) = (\hat{\delta} \hat{\Lambda} \log(m e^{-1}))^\top \quad (145)$$

Moreover, we have the following identities that involve  $Y_n$ .

$$\hat{\Lambda}^\top \hat{\delta} Y_{n-1}(\textcolor{red}{m}e^{-1}) = (\hat{\Lambda}^\top \hat{\delta} Y_{n-1}(\textcolor{red}{m}e^{-1}))^\top \quad (146)$$

$$v^\top \hat{\Lambda}^\top \hat{\delta} Y_{n-1}(\textcolor{red}{m}e^{-1}) \hat{\Lambda}^{-1} = v^\top (\hat{\Lambda}^\top \hat{\delta} Y_{n-1}(\textcolor{red}{m}e^{-1}))^\top \hat{\Lambda}^{-1} \quad (147)$$

$$= (\hat{\Lambda}^\top \hat{\delta} Y_{n-1}(\textcolor{red}{m}e^{-1})v)^\top \hat{\Lambda}^{-1} \quad (148)$$

$$= (\hat{\delta} Y_{n-1}(\textcolor{red}{m}e^{-1})v)^\top \quad (149)$$

*contd.* For the symmetric  $\hat{\delta} \hat{\Lambda} m e^{-1}$ , we have:

$$\begin{aligned} \delta \mathcal{V}^\top &= \hat{\delta} Y_{n-1}(\textcolor{red}{m}e^{-1}) \textcolor{red}{m} \left( \frac{\lambda}{\lambda+1} (\textcolor{blue}{N}e^{-1} + \textcolor{red}{M}m^{-1})v + \mu - \nu \right) \\ &\quad + \frac{1}{\lambda+1} (v^\top \hat{\Lambda}^\top \hat{\delta} Y_{n-1}(\textcolor{red}{m}e^{-1}) \textcolor{red}{m} (\textcolor{blue}{N}e^{-1} + \textcolor{red}{M}m^{-1}) \hat{\Lambda}^{-1})^\top \end{aligned} \quad (150)$$

$$\begin{aligned} &= \hat{\delta} Y_{n-1}(\textcolor{red}{m}e^{-1}) \textcolor{red}{m} \left( \frac{\lambda}{\lambda+1} (\textcolor{blue}{N}e^{-1} + \textcolor{red}{M}m^{-1})v + \mu - \nu \right) \\ &\quad + \frac{1}{\lambda+1} \hat{\delta} Y_{n-1}(\textcolor{red}{m}e^{-1}) \textcolor{red}{m} (\textcolor{blue}{N}e^{-1} + \textcolor{red}{M}m^{-1})v \end{aligned} \quad (151)$$

$$= \hat{\delta} Y_{n-1}(\textcolor{red}{m}e^{-1}) \textcolor{red}{m} ((\textcolor{blue}{N}e^{-1} + \textcolor{red}{M}m^{-1})v + \mu - \nu) \quad (152)$$

$$= \hat{\delta} Y_{n-1}(\textcolor{red}{m}e^{-1}) \textcolor{red}{m} \Delta n \quad (153)$$

**Conclusion:**  $\Delta n = 0$

The EoM for  $p = \lambda v$  yields the shift redefinition together with the spatial vielbein symmetrization (which is equivalent to the principal square root):

$$\nu = \textcolor{blue}{N}e^{-1}v + \textcolor{red}{M}m^{-1}v + \mu$$

$$\hat{\delta} \hat{\Lambda} m e^{-1} = (\hat{\delta} \hat{\Lambda} m e^{-1})^\top$$
