# Supplementary material for: Bimetric interactions based on metric congruences
Source: arXiv:1906.11841 ancillary file (2019-06-27)
Supplement: Supplementary file 2 [file bim-cong-proofs.pdf]

# Bimetric interactions based on metric congruences

Mikica Kocic, (created 2015-04-11, last modified 2019-05-16)

This notebook contains the proofs of various identities that involve elementary symmetric polynomials.

The identities are first derived by hand (incrementally, so the derivations can be tracked), then each step of the derivation is verified in *Mathematica*. All the expressions that end with “// ■ ...” are asserted to be identities in an arbitrary (random) matrix bases. Violations of the claims are reported as “△Failed△”.

The code optionally produces a **T<sub>E</sub>X code** (compiled using pdf<sub>l</sub>atex, unless in the debug mode). Clicking on the T<sub>E</sub>X output will copy the actual T<sub>E</sub>X commands to the clipboard. After evaluating the entire notebook, clicking on “Gen texOut” produces the T<sub>E</sub>X version of this document. **Note:** If you modify the notebook, do not forget to export “.tex” (which will be used as a template for “Gen texOut”).

The **toolbar** can be used to assert or T<sub>E</sub>X-out the expressions out of order.

## Changelog

2015-04-11 Unconstrained bimetric potential based on metric contgurences

2015-04-28 Identities involving symmetric polynomials

2015-05-01 Varying the potential wrt  $p$ , obtained EoM and  $\Delta n = 0$

2015-05-03 Vandermonde reparametrization

2015-05-04 Solving for symmetrizing  $\Lambda$  (the final result)

2017-12-02 Optimized the proof functions

2017-12-22 Proof functions moved to a package (to be used with the geometric mean paper)

2017-02-12 Refactoring Lorentz factor to  $\lambda$ , the shift of  $h$  to  $q$

2019-05-12 Refactoring, put hats on all spatial restrictions

2019-05-14 Split into: “definitions.nb”, “bim-cong-proofs.nb”, and “geom-mean-paper.nb”

2019-05-16 LaTeX report generator

## Load the definitions

### Notation

- $\eta$  is the Minkowski metric having signature  $(-, +, +, \dots)$ ,  $\mathbb{I}$  is the identity matrix,  $\mathbb{Z}$  denotes the zero matrix,  $\hat{\delta}$  is the spatial (Euclidean) metric,  $\hat{\mathbb{I}}$  is the spatial identity matrix, and  $\hat{\mathbb{Z}}$  is the spatial zero matrix,
- $\overset{k}{A}$  denotes the matrix power,  $A \cdot B$  denotes the matrix multiplication,  $\square$  flattens a partitioned matrix,  $\blacktriangledown$  gets the spatial part of a matrix or vector,  $\mathcal{E}_n$  denotes the elementary symmetric polynomials,  $\mathcal{Y}_n$  denotes the derivatives of  $\mathcal{E}_{n+1}$ .
- `// ■` asserts a general claim. `// ■n` asserts a claim for any  $n$ . `// ■$X` asserts claims for an arbitrary  $d$ -dimensional matrix  $X$ . `// ■$D` asserts claims for an arbitrary  $(d-1)$ -dimensional matrix  $D$ . `// ■$v` asserts claims for an arbitrary  $(d-1)$ -dimensional vector  $v$  (not restricted to  $v^2 < 1$ ). `// ■$Nen` and `// ■$Ndet` assert the expressions claimed to be equal to  $N\mathcal{E}_n[S]$  and  $N\det[S] \mathcal{E}_n[S]$ , respectively.

## Part I

## Propositions involving $e_n$ and $Y_n$

The following claims hold for an arbitrary  $d$ -dimensional matrix  $X$ .

### Partition of ESP

In[1]:=

```
 $\mathcal{E}_d[X] \mathcal{E}_n[\bar{X}^1] == \mathcal{E}_{d-n}[X] // \blacksquare X$ 
```

True

True

True

True

True

True

## Recursive relation for $Y_n(X) = \partial e_{n+1}(X) / \partial X^T$

$$\text{In[2]: } Y_n[X] == \sum_{k=0}^n (-1)^{n+k} \mathcal{E}_k[X] X^{n-k} // \blacksquare X$$

True True True True True True

$$\text{In[3]: } Y_0[X] == I // \blacksquare X$$

True True True True True True

$$\text{In[4]: } Y_{-1}[X] == Z // \blacksquare X$$

True True True True True True

$$\text{In[5]: } Y_n[X] == \mathcal{E}_n[X] I - X \cdot Y_{n-1}[X] // \blacksquare X$$

True True True True True True

## Damour's algebraic identity

$$\text{In[6]: } Yf_n[X] == \sum_{k=0}^{d-n} (-1)^{d-n+k} \mathcal{E}_k[X^{-1}] X^{-(d-n-k)} // \blacksquare X$$

True True True True True True

$$\text{In[7]: } Yf_0[X] == Z // \blacksquare X$$

True True True True True True

$$\text{In[8]: } Yf_{-1}[X] == Z // \blacksquare X$$

True True True True True True

$$\text{In[9]: } Yf_n[X] == Y_{d-n}[X^{-1}] // \blacksquare X$$

True True True True True True

$$\text{In[10]: } Y_n[X] + \mathcal{E}_d[X] Y_{d-n}[X^{-1}] == \mathcal{E}_n[X] I // \blacksquare X$$

True True True True True True

$$\text{In[11]: } Y_n[X] + \text{Det}[X] Yf_n[X] == \mathcal{E}_n[X] I // \blacksquare X$$

True True True True True True

## Identities involving the projections $e_n(I + UW^T)$

Here,  $U$  and  $W$  are  $d$ -dimensional column vectors. Matrices having the form  $I + UW^T$  are part of the Lorentz transformations, the square roots and the projections.

$$\text{In[12]: } n \mathcal{E}_n[X] == \sum_{k=1}^n (-1)^{k-1} \mathcal{E}_{n-k}[X] \text{Tr}[X^k] // \blacksquare X$$

True True True True True True

$$\text{In[13]: } \mathcal{E}_n[X + U \cdot W^T] == \text{If}[n == 0, 1, \sum_{k=1}^n (-1)^{k-1} \mathcal{E}_{n-k}[X] \text{Tr}[X^{k-1} \cdot \left(\frac{1}{n} X + U \cdot W^T\right)]] // \blacksquare X$$

True True True True True True

$$\text{In[14]}:= \mathcal{E}_n[\mathbf{X} + \mathbf{U} \cdot \mathbf{W}^T] == \mathcal{E}_n[\mathbf{X}] + \sum_{k=1}^n (-1)^{k-1} \mathcal{E}_{n-k}[\mathbf{X}] \mathbf{W}^T \cdot \overset{k-1}{\mathbf{X}} \cdot \mathbf{U} // \blacksquare \$\mathbf{X}$$

True True True True True True

$$\text{In[15]}:= \mathcal{E}_n[\mathbf{X} \cdot (\mathbb{I} + \mathbf{U} \cdot \mathbf{W}^T)] == \mathcal{E}_n[\mathbf{X}] + \sum_{k=1}^n (-1)^{k-1} \mathcal{E}_{n-k}[\mathbf{X}] \mathbf{W}^T \cdot \overset{k}{\mathbf{X}} \cdot \mathbf{U} // \blacksquare \$\mathbf{X}$$

True True True True True True

$$\text{In[16]}:= \mathcal{E}_n[\mathbf{X} \cdot (\mathbb{I} + \mathbf{U} \cdot \mathbf{W}^T)] == \mathcal{E}_n[\mathbf{X}] + \mathbf{W}^T \cdot \mathbf{X} \cdot \sum_{k=0}^{n-1} (-1)^{n-1+k} \mathcal{E}_k[\mathbf{X}] \overset{n-1-k}{\mathbf{X}} \cdot \mathbf{U} // \blacksquare \$\mathbf{X}$$

True True True True True True

$$\text{In[17]}:= (* \text{ use: } *) \mathbf{Y}_n[\mathbf{X}] == \sum_{k=0}^n (-1)^{n+k} \mathcal{E}_k[\mathbf{X}] \overset{n-k}{\mathbf{X}} // \blacksquare \$\mathbf{X}$$

True True True True True True

$$\text{In[18]}:= \mathcal{E}_n[\mathbf{X} \cdot (\mathbb{I} + \mathbf{U} \cdot \mathbf{W}^T)] == \mathcal{E}_n[\mathbf{X}] + \mathbf{W}^T \cdot \mathbf{X} \cdot \mathbf{Y}_{n-1}[\mathbf{X}] \cdot \mathbf{U} // \blacksquare \$\mathbf{X}$$

True True True True True True

$$\text{In[19]}:= \mathcal{E}_n[\mathbf{X} \cdot (\mathbb{I} + \mathbf{U} \cdot \mathbf{W}^T)] == \mathcal{E}_n[\mathbf{X}] + \mathbf{W}^T \cdot (\mathcal{E}_n[\mathbf{X}] \mathbb{I} - \mathbf{Y}_n[\mathbf{X}]) \cdot \mathbf{U} // \blacksquare \$\mathbf{X}$$

True True True True True True

$$\text{In[20]}:= \mathcal{E}_n[\mathbf{X} \cdot (\mathbb{I} + \mathbf{U} \cdot \mathbf{W}^T)] == \mathcal{E}_n[\mathbf{X}] (1 + \mathbf{W}^T \cdot \mathbf{U}) - \mathbf{W}^T \cdot \mathbf{Y}_n[\mathbf{X}] \cdot \mathbf{U} // \blacksquare \$\mathbf{X}$$

True True True True True True

$$\text{In[21]}:= \mathcal{E}_n[\mathbf{X} + \mathbf{U} \cdot \mathbf{W}^T] == \mathcal{E}_n[\mathbf{X}] + \sum_{k=1}^n (-1)^{k-1} \mathcal{E}_{n-k}[\mathbf{X}] \mathbf{W}^T \cdot \overset{k-1}{\mathbf{X}} \cdot \mathbf{U} // \blacksquare \$\mathbf{X}$$

True True True True True True

$$\text{In[22]}:= \mathcal{E}_n[\mathbf{X} + \mathbf{U} \cdot \mathbf{W}^T] == \mathcal{E}_n[\mathbf{X}] + \sum_{k=0}^{n-1} (-1)^{n-1+k} \mathcal{E}_k[\mathbf{X}] \mathbf{W}^T \cdot \overset{n-1-k}{\mathbf{X}} \cdot \mathbf{U} // \blacksquare \$\mathbf{X}$$

True True True True True True

$$\text{In[23]}:= \mathcal{E}_n[\mathbf{X} + \mathbf{U} \cdot \mathbf{W}^T] == \mathcal{E}_n[\mathbf{X}] + \mathbf{W}^T \cdot \mathbf{Y}_{n-1}[\mathbf{X}] \cdot \mathbf{U} // \blacksquare \$\mathbf{X}$$

True True True True True True

$$\text{In[24]}:= \mathcal{E}_n[\mathbf{X} + \mathbf{U} \cdot \mathbf{W}^T] == \mathcal{E}_n[\mathbf{X}] + \mathbf{W}^T \cdot (\mathcal{E}_{n-1}[\mathbf{X}] \mathbb{I} - \mathbf{X} \cdot \mathbf{Y}_{n-2}[\mathbf{X}]) \cdot \mathbf{U} // \blacksquare \$\mathbf{X}$$

True True True True True True

$$\text{In[25]}:= \mathcal{E}_n[\mathbf{X} + \mathbf{U} \cdot \mathbf{W}^T] == \mathcal{E}_n[\mathbf{X}] + \mathcal{E}_{n-1}[\mathbf{X}] \mathbf{W}^T \cdot \mathbf{U} - \mathbf{W}^T \cdot \mathbf{X} \cdot \mathbf{Y}_{n-2}[\mathbf{X}] \cdot \mathbf{U} // \blacksquare \$\mathbf{X}$$

True True True True True True

## Cayley-Hamilton theorem and the related identities

The following claims hold for an arbitrary  $(d-1)$ -dimensional matrix  $D$ .

$$\text{In}[26]:= \sum_{k=0}^d (-1)^{d-k} \boxed{\mathcal{E}_{d-k}[D]} \overset{k}{D} = 0 \quad // \quad \blacksquare \$D$$

True True True True True True

$$\text{In}[27]:= \sum_{k=0}^{d-1} (-1)^{d-1-k} \boxed{\mathcal{E}_{d-1-k}[D]} \overset{k}{D} = 0 \quad // \quad \blacksquare \$D$$

True True True True True True

$$\text{In}[28]:= \sum_{k=1}^{d-n} (-1)^{k-1} \boxed{\mathcal{E}_{d-n-k}[D]} \overset{k}{D} = \left( \sum_{k=n+1}^d (-1)^{k-(n+1)} \boxed{\mathcal{E}_{d-k}[D]} \overset{k-n}{D} \right) \quad // \quad \blacksquare \$D$$

True True True True True True

$$\text{In}[29]:= \sum_{k=1}^{d-n} (-1)^{k-1} \boxed{\mathcal{E}_{d-n-k}[D]} \overset{k}{D} = \left( \sum_{k=n+1}^d (-1)^{k-(n+1)} \boxed{\mathcal{E}_{d-k}[D]} \overset{k}{D} \cdot \overset{-n}{D} \right) \quad // \quad \blacksquare \$D$$

True True True True True True

$$\text{In}[30]:= \sum_{k=1}^{d-n} (-1)^{k-1} \boxed{\mathcal{E}_{d-n-k}[D]} \overset{k}{D} = \left( \sum_{k=n}^{d-1} (-1)^{k-n} \boxed{\mathcal{E}_{d-1-k}[D]} \overset{k}{D} \cdot \overset{-n+1}{D} \right) \quad // \quad \blacksquare \$D$$

True True True True True True

$$\text{In}[31]:= \sum_{k=1}^{d-n} (-1)^{k-1} \boxed{\mathcal{E}_{d-n-k}[D]} \overset{k}{D} = \left( - \sum_{k=0}^{n-1} (-1)^{k-n} \boxed{\mathcal{E}_{d-1-k}[D]} \overset{k}{D} \cdot \overset{-n+1}{D} \right) \quad // \quad \blacksquare \$D$$

True True True True True True

$$\text{In}[32]:= \sum_{k=1}^{d-n} (-1)^{k-1} \boxed{\mathcal{E}_{d-n-k}[D]} \overset{k}{D} = \left( -\text{Det}[D] \sum_{k=0}^{n-1} (-1)^{k-n} \boxed{\mathcal{E}_k[\overset{-1}{D}]} \overset{k}{D} \cdot \overset{-n+1}{D} \right) \quad // \quad \blacksquare \$D$$

True True True True True True

$$\text{In}[33]:= \sum_{k=1}^{d-n} (-1)^{k-1} \boxed{\mathcal{E}_{d-n-k}[D]} \overset{k}{D} = \left( -\text{Det}[D] \sum_{k=0}^{n-1} (-1)^{n-1-k-n} \boxed{\mathcal{E}_{n-1-k}[\overset{-1}{D}]} \overset{n-1-k}{D} \cdot \overset{-n+1}{D} \right) \quad // \quad \blacksquare \$D$$

True True True True True True

$$\text{In}[34]:= \sum_{k=1}^{d-n} (-1)^{k-1} \boxed{\mathcal{E}_{d-n-k}[D]} \overset{k}{D} = \left( -\text{Det}[D] \sum_{k=1}^n (-1)^{n-k-n} \boxed{\mathcal{E}_{n-k}[\overset{-1}{D}]} \overset{n-k}{D} \cdot \overset{-n+1}{D} \right) \quad // \quad \blacksquare \$D$$

True True True True True True

$$\text{In}[35]:= \sum_{k=1}^{d-n} (-1)^{k-1} \boxed{\mathcal{E}_{d-n-k}[D]} \overset{k}{D} = \text{Det}[D] \left( \sum_{k=1}^n (-1)^{k-1} \boxed{\mathcal{E}_{n-k}[\overset{-1}{D}]} \overset{-(k-1)}{D} \right) \quad // \quad \blacksquare \$D$$

True True True True True True

# Lorentz transformation $\Lambda$

The following claims hold for an arbitrary  $(d-1)$ -dimensional vector  $\mathbf{v}$  (not restricted to  $|\mathbf{v}| < 1$ ).

$$\text{In[36]:= } \boldsymbol{\eta} == \overline{\boldsymbol{\Lambda}}^T \cdot \boldsymbol{\eta} \cdot \overline{\boldsymbol{\Lambda}} // \blacksquare \$\mathbf{v}$$

True

$$\text{In[37]:= } \overline{\boldsymbol{\Lambda}} == \square \begin{pmatrix} \lambda & \mathbf{p}^T \cdot \hat{\boldsymbol{\delta}} \\ \mathbf{p} & \hat{\boldsymbol{\Lambda}} \end{pmatrix} // \blacksquare \$\mathbf{v}$$

True

$$\text{In[38]:= } \mathbf{p} == \lambda \mathbf{v} // \blacksquare \$\mathbf{v}$$

True

## The temporal part of $\Lambda$

$$\text{In[39]:= } \lambda^2 == (1 + \mathbf{p}^T \cdot \hat{\boldsymbol{\delta}} \cdot \mathbf{p}) == \frac{1}{1 - \mathbf{v}^T \cdot \hat{\boldsymbol{\delta}} \cdot \mathbf{v}} // \blacksquare \$\mathbf{v}$$

True

True

## The spatial part of $\Lambda$

$$\text{In[40]:= } \hat{\boldsymbol{\Lambda}} == \hat{\mathbf{I}} + \frac{\lambda^2}{\lambda + 1} \mathbf{v} \cdot \mathbf{v}^T \cdot \hat{\boldsymbol{\delta}} // \blacksquare \$\mathbf{v}$$

True

$$\text{In[41]:= } \hat{\boldsymbol{\Lambda}}^2 == (\hat{\mathbf{I}} + \mathbf{p} \cdot \mathbf{p}^T \cdot \hat{\boldsymbol{\delta}}) == (\hat{\mathbf{I}} + \lambda^2 \mathbf{v} \cdot \mathbf{v}^T \cdot \hat{\boldsymbol{\delta}}) // \blacksquare \$\mathbf{v}$$

True

True

$$\text{In[42]:= } \hat{\boldsymbol{\Lambda}}^{-1} == \left( \hat{\mathbf{I}} - \frac{\lambda}{\lambda + 1} \mathbf{v} \cdot \mathbf{v}^T \cdot \hat{\boldsymbol{\delta}} \right) == \left( \hat{\mathbf{I}} - \frac{1}{\lambda (\lambda + 1)} \mathbf{p} \cdot \mathbf{p}^T \cdot \hat{\boldsymbol{\delta}} \right) // \blacksquare \$\mathbf{v}$$

True

True

$$\text{In[43]:= } \hat{\boldsymbol{\Lambda}}^{-2} == (\hat{\mathbf{I}} - \mathbf{v} \cdot \mathbf{v}^T \cdot \hat{\boldsymbol{\delta}}) == (\hat{\mathbf{I}} - \lambda^{-2} \mathbf{p} \cdot \mathbf{p}^T \cdot \hat{\boldsymbol{\delta}}) // \blacksquare \$\mathbf{v}$$

True

True

$$\text{In[44]:= } \hat{\boldsymbol{\delta}} \cdot \hat{\boldsymbol{\Lambda}} == (\hat{\boldsymbol{\delta}} \cdot \hat{\boldsymbol{\Lambda}})^T == \hat{\boldsymbol{\Lambda}}^T \cdot \hat{\boldsymbol{\delta}} // \blacksquare$$

True

True

## The eigenvalues (all but one are 1)

$$\text{In[45]:= } \hat{\boldsymbol{\Lambda}} \cdot \mathbf{v} == \lambda \mathbf{v} // \blacksquare \$\mathbf{v}$$

True

$$\text{In[46]:= } \text{Det}@\hat{\boldsymbol{\Lambda}} == \lambda // \blacksquare \$\mathbf{v}$$

True

## Part 2

### Setup the metrics and verify relations between the variables

#### Metrics, vielbeins, and spatial metrics

In[47]:= `random$g[]; g == ET · η · E //` ■

True

In[48]:= `random$f[]; f == LT · η · L //` ■

True

In[49]:= `ĝ == ∇@g //` ■

True

In[50]:= `f̂ == ∇@f //` ■

True

#### Vielbeins

In[51]:= `E == □ (  $\begin{pmatrix} \mathbf{N} & 0 \\ \mathbf{e} \cdot \mathbf{v} & \mathbf{e} \end{pmatrix}$  ) //` ■

True

In[52]:= `L == □ (  $\begin{pmatrix} \mathbf{u}0 + \mathbf{u}^T \cdot \mathbf{q} & \mathbf{u}^T \\ \hat{\mathbf{L}} \cdot \mathbf{q} & \hat{\mathbf{L}} \end{pmatrix}$  ) == □ (  $\begin{pmatrix} \lambda & \lambda \mathbf{v}^T \cdot \hat{\boldsymbol{\delta}} \\ \lambda \mathbf{v} & \hat{\boldsymbol{\Lambda}} \end{pmatrix}$  ) · □ (  $\begin{pmatrix} \mathbf{M} & 0 \\ \mathbf{m} \cdot \boldsymbol{\mu} & \mathbf{m} \end{pmatrix}$  ) //` ■

True

True

#### General parametrization of the vielbein L

In[53]:= `L̂ == Λ̂ · m //` ■

True

In[54]:= `u0 == λ-1 M //` ■

True

In[55]:= `u == (  $\mathbf{v}^T \cdot \hat{\boldsymbol{\delta}} \cdot \hat{\boldsymbol{\Lambda}} \cdot \mathbf{m}$  )T //` ■

True

In[56]:= `q == M  $\hat{\mathbf{m}}^{-1}$  · v + μ //` ■

True

In[57]:= `f̂ == -u · uT + L̂T · δ̂ · L̂ //` ■

True

## The $N + 1$ decomposition of the vielbein $L$

In[58]:=  $\mathbf{M} == \lambda \mathbf{u} \mathbf{0} // \blacksquare$

True

In[59]:=  $\mathbf{m} == \hat{\mathbf{A}}^{-1} \cdot \hat{\mathbf{L}} // \blacksquare$

True

In[60]:=  $\mu == \mathbf{q} - \mathbf{M} \hat{\mathbf{m}}^{-1} \cdot \mathbf{v} // \blacksquare$

True

In[61]:=  $\mathbf{v} == \left( \mathbf{u}^\top \cdot \hat{\mathbf{L}}^{-1} \cdot \hat{\delta} \right)^\top // \blacksquare$

True

Check if the vielbein  $L$  is a proper one,

In[62]:=  $\text{If}[\text{ValueQ}[\mathbf{g}] \wedge (\text{Norm}[\mathbf{v}] \geq 1 \vee \text{Im}@\mathbf{M} \neq 0 \vee \text{Not}@\text{PositiveDefiniteMatrixQ}@\hat{\mathbf{f}}),$   
 $\text{Print}[|\mathbf{v}| = , \text{Norm}[\mathbf{v}], "\backslash n",$   
 $"\mathbf{M} = ", \mathbf{M}, "\backslash n",$   
 $"\hat{\mathbf{f}} \text{ positive definite: ", PositiveDefiniteMatrixQ}@\hat{\mathbf{f}}$   
 $], \text{If}[\text{ValueQ}[\mathbf{g}], \mathbf{v}^\top \cdot \hat{\delta} \cdot \mathbf{v} < 1, \mathbf{v}^\top \cdot \hat{\delta} \cdot \mathbf{v} < 1 // \blacksquare]]$

Out[62]= True

## At this point, we do not have a square root (!)

In[63]:=  $\Delta \mathbf{n} == \left( \mathbf{N} \hat{\mathbf{e}}^{-1} + \mathbf{M} \hat{\mathbf{m}}^{-1} \right) \cdot \mathbf{v} + \mu - \mathbf{v} // \blacksquare$

True

In[64]:=  $\Delta \mathbf{n} \neq 0 // \blacksquare$

True

In[65]:=  $\hat{\delta} \cdot \hat{\mathbf{A}} \cdot \left( \mathbf{m} \cdot \hat{\mathbf{e}}^{-1} \right) \neq \left( \hat{\delta} \cdot \hat{\mathbf{A}} \cdot \left( \mathbf{m} \cdot \hat{\mathbf{e}}^{-1} \right) \right)^\top // \blacksquare$

True

## Congruence $\hat{\mathbf{B}}$ (where $\hat{\mathbf{B}}$ is the spatial part of $\mathbf{s}$ that is pulled by $\mathbf{e}$ )

In[66]:=  $\hat{\mathbf{B}} == \hat{\mathbf{e}}^{-1} \cdot \hat{\mathbf{A}} \cdot \mathbf{m} == \hat{\mathbf{e}}^{-1} \cdot \hat{\mathbf{L}} // \blacksquare$

True

True

In[67]:=  $\hat{\mathbf{B}}^\top \cdot \hat{\mathbf{g}} \cdot \hat{\mathbf{B}} == \hat{\mathbf{L}}^\top \cdot \hat{\delta} \cdot \hat{\mathbf{L}} == \hat{\mathbf{f}} + \mathbf{u} \cdot \mathbf{u}^\top // \blacksquare$

True

True

## Lorentz transformation in terms of $f$

In[68]:=  $\lambda^{-2} == \mathbf{x} // \blacksquare$

True

$$\text{In[69]:= } \mathbf{Q} == \hat{\mathbf{m}}^{-1} \cdot \hat{\mathbf{A}} \cdot \hat{\mathbf{A}} \cdot \mathbf{m} == (\hat{\mathbf{f}} + \lambda^2 \mathbf{m} \cdot \mathbf{m}^T \cdot \hat{\mathbf{f}}) // \blacksquare$$

True True

$$\text{In[70]:= } \hat{\mathbf{f}} \cdot \mathbf{Q} == \mathbf{Q}^T \cdot \hat{\mathbf{f}} // \blacksquare$$

True

$$\text{In[71]:= } \hat{\mathbf{B}}^T \cdot \hat{\mathbf{g}} \cdot \hat{\mathbf{B}} == \hat{\mathbf{f}} \cdot \mathbf{Q} == \hat{\mathbf{f}} + \mathbf{u} \cdot \mathbf{u}^T // \blacksquare$$

True True

## Relations between $\hat{\mathbf{D}}$ and $\hat{\mathbf{B}}$

$$\text{In[72]:= } \hat{\mathbf{B}} == \hat{\mathbf{D}} \cdot \mathbf{Q} // \blacksquare$$

True

$$\text{In[73]:= } \hat{\mathbf{D}} \hat{\mathbf{g}} == \hat{\mathbf{Q}}^{-1} \cdot \hat{\mathbf{D}}^{-1} // \blacksquare$$

True

## The determinants of $\mathbf{S}$ , $\hat{\mathbf{D}}$ and $\hat{\mathbf{B}}$

$$\text{In[74]:= } \text{Det@S} == \mathcal{E}_d[\mathbf{S}] // \blacksquare$$

True

$$\text{In[75]:= } \triangleleft == \mathcal{E}_d[\hat{\mathbf{D}}] + \frac{\mathbf{M}}{\mathbf{N} \lambda} \mathcal{E}_{d-1}[\hat{\mathbf{B}}] == \frac{\mathbf{M}}{\mathbf{N} \lambda} \mathcal{E}_{d-1}[\hat{\mathbf{B}}] // \blacksquare$$

True True

$$\text{In[76]:= } \triangleleft == \frac{\mathbf{M}}{\mathbf{N} \lambda} \text{Det}[\hat{\mathbf{B}}] == \frac{\mathbf{M}}{\mathbf{N} \lambda} \text{Det}[\hat{\mathbf{D}} \cdot \mathbf{Q}] // \blacksquare$$

True True

$$\text{In[77]:= } \text{Det}[\mathbf{Q}] == \lambda^2 // \blacksquare$$

True

$$\text{In[78]:= } \text{Det@S} == \frac{\mathbf{M} \lambda}{\mathbf{N}} \text{Det}[\hat{\mathbf{D}}] // \blacksquare$$

True

$$\text{In[79]:= } \frac{1}{\text{Det@S}} == \frac{\mathbf{N}}{\mathbf{M} \lambda} \text{Det}[\hat{\mathbf{D}}^{-1}] // \blacksquare$$

True

## The decomposition of $e_n(S)$

The identities below are modified step-by-step (with minimal changes between two consecutive equations). The derivations are done in several branches. The last branch contains the expression for  $Ne_n(S)$  that is varied to get EoM.

The main expressions equal to  $Ne_n(S)$

$$\text{In[80]:= } \text{If}[\text{Not@ValueQ}[\mathbf{g}], \text{Text}["\text{Established } "] \mathbf{N} \mathcal{E}_n[\mathbf{S}] \text{Text}[" : "] // \blacksquare$$



$$\text{In}[81]:= \mathbf{N} \left[ \mathcal{E}_n[\hat{\mathbf{B}}] \right] + \mathbf{u} \mathbf{0} \left[ \mathcal{E}_{n-1}[\hat{\mathbf{B}}] \right] + \sum_{k=1}^n (-1)^{k-1} \left[ \mathcal{E}_{n-k}[\hat{\mathbf{B}}] \right] \mathbf{u}^\top \cdot \hat{\mathbf{B}}^{k-1} \cdot (\mathbf{q} - \mathbf{v}) // \blacksquare \$\mathbf{N} \mathbf{E} n$$

True True True True True True

$$\text{In}[82]:= \mathbf{N} \left[ \mathcal{E}_n[\hat{\mathbf{D}}] \right] + \mathbf{u} \mathbf{0} \left[ \mathcal{E}_{n-1}[\hat{\mathbf{B}}] \right] + \sum_{k=1}^n (-1)^{k-1} \left[ \mathcal{E}_{n-k}[\hat{\mathbf{B}}] \right] \mathbf{u}^\top \cdot \hat{\mathbf{B}}^{k-1} \cdot \Delta n // \blacksquare \$\mathbf{N} \mathbf{E} n$$

True True True True True True

$$\text{In}[83]:= \mathbf{N} \left[ \mathcal{E}_n[\hat{\mathbf{D}}] \right] + \mathbf{u} \mathbf{0} \left[ \mathcal{E}_{n-1}[\hat{\mathbf{B}}] \right] + \left[ \mathcal{E}_n[\hat{\mathbf{B}} + \Delta n \cdot \mathbf{u}^\top] \right] - \left[ \mathcal{E}_n[\hat{\mathbf{B}}] \right] // \blacksquare \$\mathbf{N} \mathbf{E} n$$

True True True True True True

$$\text{In}[84]:= \mathbf{N} \left[ \mathcal{E}_n[\hat{\mathbf{B}}] \right] + \lambda^{-1} \mathbf{M} \left[ \mathcal{E}_{n-1}[\hat{\mathbf{B}}] \right] + \lambda \sum_{k=1}^n (-1)^{k-1} \left[ \mathcal{E}_{n-k}[\hat{\mathbf{B}}] \right] \mathbf{m}^\top \cdot \hat{\mathbf{f}} \cdot \hat{\mathbf{B}}^{k-1} \cdot (\mathbf{q} - \mathbf{v}) // \blacksquare \$\mathbf{N} \mathbf{E} n$$

True True True True True True

$$\text{In}[85]:= \mathbf{N} \left[ \mathcal{E}_n[\hat{\mathbf{D}}] \right] + \lambda^{-1} \mathbf{M} \left[ \mathcal{E}_{n-1}[\hat{\mathbf{B}}] \right] + \lambda \sum_{k=1}^n (-1)^{k-1} \left[ \mathcal{E}_{n-k}[\hat{\mathbf{B}}] \right] \mathbf{m}^\top \cdot \hat{\mathbf{f}} \cdot \hat{\mathbf{B}}^{k-1} \cdot \Delta n // \blacksquare \$\mathbf{N} \mathbf{E} n$$

True True True True True True

$$\text{In}[86]:= \mathbf{N} \text{Det}[\mathbf{e}] \left[ \mathcal{E}_n[\hat{\mathbf{D}}] \right] + \mathbf{M} \text{Det}[\mathbf{m}] \left[ \mathcal{E}_{d-n}[\hat{\mathbf{D}}\mathbf{g}] \right] + \text{Det}[\mathbf{e}] \sum_{k=1}^n (-1)^{k-1} \left[ \mathcal{E}_{n-k}[\hat{\mathbf{B}}] \right] \lambda \mathbf{m}^\top \cdot \hat{\mathbf{f}} \cdot \hat{\mathbf{B}}^{k-1} \cdot \Delta n // \blacksquare \$\mathbf{N} \mathbf{D} \mathbf{E} n$$

True True True True True True

**Strategy:** We should rewrite  $Ne_n(S)$  to obtain the equations that contain an isolated  $p$  together with the elementary symmetric polynomials which are of the form  $Ne_n(me^{-1})$  or  $Ne_n(em^{-1})$ .

## $Ne_n(S)$ Derivation track 1

$$\text{In}[87]:= \mathbf{N} \left[ \mathcal{E}_n[\hat{\mathbf{e}}^{-1} \cdot \hat{\mathbf{A}} \cdot \mathbf{m}] \right] + \lambda^{-1} \mathbf{M} \left[ \mathcal{E}_{n-1}[\hat{\mathbf{e}}^{-1} \cdot \hat{\mathbf{A}} \cdot \mathbf{m}] \right] - \left[ \mathcal{E}_n[\hat{\mathbf{B}}] \right] +$$

$$\text{[RET]} + \left[ \mathcal{E}_n[\hat{\mathbf{e}}^{-1} \cdot \hat{\mathbf{A}} \cdot \mathbf{m} + (\mathbf{M} \hat{\mathbf{m}}^{-1} \cdot \mathbf{v} + \mu - \mathbf{v}) \cdot \mathbf{v}^\top \cdot \hat{\delta} \cdot \hat{\mathbf{A}} \cdot \mathbf{m}] \right] // \blacksquare \$\mathbf{N} \mathbf{E} n$$

True True True True True True

$$\text{In}[88]:= \mathbf{N} \left[ \mathcal{E}_n[\hat{\mathbf{e}}^{-1} \cdot \hat{\mathbf{A}} \cdot \mathbf{m}] \right] + \lambda^{-1} \mathbf{M} \left[ \mathcal{E}_{n-1}[\hat{\mathbf{e}}^{-1} \cdot \hat{\mathbf{A}} \cdot \mathbf{m}] \right] - \left[ \mathcal{E}_n[\hat{\mathbf{e}}^{-1} \cdot \hat{\mathbf{A}} \cdot \mathbf{m} - \mathbf{M} \hat{\mathbf{m}}^{-1} \cdot \mathbf{v} \cdot \mathbf{v}^\top \cdot \hat{\delta} \cdot \hat{\mathbf{A}} \cdot \mathbf{m}] \right] +$$

$$\text{[RET]} + \left[ \mathcal{E}_n[\hat{\mathbf{e}}^{-1} \cdot \hat{\mathbf{A}} \cdot \mathbf{m} + (\mu - \mathbf{v}) \cdot \mathbf{v}^\top \cdot \hat{\delta} \cdot \hat{\mathbf{A}} \cdot \mathbf{m}] \right] // \blacksquare \$\mathbf{N} \mathbf{E} n$$

True True True True True True

$$\text{In}[89]:= \mathbf{N} \left[ \mathcal{E}_n[\mathbf{m} \cdot \hat{\mathbf{e}}^{-1} \cdot \hat{\mathbf{A}}] \right] + \lambda^{-1} \mathbf{M} \left[ \mathcal{E}_{n-1}[\mathbf{m} \cdot \hat{\mathbf{e}}^{-1} \cdot \hat{\mathbf{A}}] \right] - \left[ \mathcal{E}_n[\mathbf{m} \cdot \hat{\mathbf{e}}^{-1} \cdot \hat{\mathbf{A}} - \lambda \mathbf{M} \mathbf{v} \cdot \mathbf{v}^\top \cdot \hat{\delta}] \right] +$$

$$\text{[RET]} + \left[ \mathcal{E}_n[\mathbf{m} \cdot \hat{\mathbf{e}}^{-1} \cdot \hat{\mathbf{A}} + \lambda \mathbf{m} \cdot (\mu - \mathbf{v}) \cdot \mathbf{v}^\top \cdot \hat{\delta}] \right] // \blacksquare \$\mathbf{N} \mathbf{E} n$$

True True True True True True



$$\text{In[99]} := \mathbf{N} \left[ \mathcal{E}_n[\hat{\mathbf{B}}] \right] + \lambda^{-1} \mathbf{M} \left[ \mathcal{E}_{n-1}[\hat{\mathbf{B}}] \right] + \lambda \left[ \mathcal{E}_n[\hat{\mathbf{B}} + (\mu - \nu) \cdot \mathbf{m}^\top \cdot \hat{\mathbf{f}}] \right] - \lambda \left[ \mathcal{E}_n[\hat{\mathbf{B}}] \right] +$$

$$\boxed{\text{RET}} + \lambda^{-1} \mathbf{M} \left[ \mathcal{E}_n[\hat{\mathbf{B}} + \lambda^2 \bar{\mathbf{m}}^{-1} \cdot \mathbf{v} \cdot \mathbf{m}^\top \cdot \hat{\mathbf{f}}] \right] - \lambda^{-1} \mathbf{M} \left[ \mathcal{E}_n[\hat{\mathbf{B}}] \right] // \blacksquare \text{\$NEn}$$

True True True True True True

$$\text{In[100]} := \mathbf{N} \left[ \mathcal{E}_n[\hat{\mathbf{B}}] \right] + \lambda^{-1} \mathbf{M} \left[ \mathcal{E}_{n-1}[\hat{\mathbf{B}}] \right] + \left[ \mathcal{E}_n[\hat{\mathbf{B}} + \lambda (\mu - \nu) \cdot \mathbf{m}^\top \cdot \hat{\mathbf{f}}] \right] - \left[ \mathcal{E}_n[\hat{\mathbf{B}} - \lambda \mathbf{M} \bar{\mathbf{m}}^{-1} \cdot \mathbf{v} \cdot \mathbf{m}^\top \cdot \hat{\mathbf{f}}] \right] // \blacksquare \text{\$NEn}$$

True True True True True True

### $\text{Ndet}(e) e_n(S)$ Derivation track 3

$$\text{In[101]} := \mathbf{N} \text{Det}[\mathbf{e}] \mathcal{E}_n[\mathbf{S}] // \blacksquare \text{\$NdEn}$$

True True True True True True

$$\text{In[102]} := \mathbf{M} \text{Det}[\mathbf{m}] \mathcal{E}_{d-n}[\bar{\mathbf{S}}] // \blacksquare \text{\$NdEn}$$

True True True True True True

$$\text{In[103]} := \mathbf{N} \text{Det}[\mathbf{e}] \left[ \mathcal{E}_n[\bar{\mathbf{e}}^{-1} \cdot \bar{\hat{\Lambda}}^{-1} \cdot \mathbf{m}] \right] + \mathbf{M} \text{Det}[\mathbf{m}] \left[ \mathcal{E}_{d-n}[\bar{\mathbf{m}}^{-1} \cdot \bar{\hat{\Lambda}}^{-1} \cdot \mathbf{e}] \right] - \text{Det}[\mathbf{e}] \left[ \mathcal{E}_n[\bar{\mathbf{e}}^{-1} \cdot \hat{\Lambda} \cdot \mathbf{m}] \right] +$$

$$\boxed{\text{RET}} + \text{Det}[\mathbf{e}] \left[ \mathcal{E}_n[\bar{\mathbf{e}}^{-1} \cdot \hat{\Lambda} \cdot \mathbf{m} + (\mathbf{N} \bar{\mathbf{e}}^{-1} \cdot \mathbf{v} + \mathbf{M} \bar{\mathbf{m}}^{-1} \cdot \mathbf{v} + \mu - \nu) \cdot \mathbf{v}^\top \cdot \hat{\delta} \cdot \hat{\Lambda} \cdot \mathbf{m}] \right] // \blacksquare \text{\$NdEn}$$

True True True True True True

$$\text{In[104]} := \mathbf{M} \text{Det}[\mathbf{m}] \left[ \mathcal{E}_{d-n}[\bar{\mathbf{m}}^{-1} \cdot \bar{\hat{\Lambda}}^{-1} \cdot \mathbf{e}] \right] + \mathbf{N} \text{Det}[\mathbf{e}] \left[ \mathcal{E}_n[\bar{\mathbf{e}}^{-1} \cdot \bar{\hat{\Lambda}}^{-1} \cdot \mathbf{m}] \right] - \text{Det}[\mathbf{m}] \left[ \mathcal{E}_{d-n}[\bar{\mathbf{m}}^{-1} \cdot \hat{\Lambda} \cdot \mathbf{e}] \right] +$$

$$\boxed{\text{RET}} + \text{Det}[\mathbf{m}] \left[ \mathcal{E}_{d-n}[\bar{\mathbf{m}}^{-1} \cdot \hat{\Lambda} \cdot \mathbf{e} + (\mathbf{N} \bar{\mathbf{e}}^{-1} \cdot \mathbf{v} + \mathbf{M} \bar{\mathbf{m}}^{-1} \cdot \mathbf{v} + \mu - \nu) \cdot \mathbf{v}^\top \cdot \hat{\delta} \cdot \hat{\Lambda} \cdot \mathbf{e}] \right] // \blacksquare \text{\$NdEn}$$

True True True True True True

$$\text{In[105]} := \boxed{\text{TAB}} \text{Det}[\mathbf{e}] \left( \left[ \mathcal{E}_n[\bar{\mathbf{e}}^{-1} \cdot \hat{\Lambda} \cdot \mathbf{m} + (\mathbf{N} \bar{\mathbf{e}}^{-1} \cdot \mathbf{v} + \mathbf{M} \bar{\mathbf{m}}^{-1} \cdot \mathbf{v} + \mu - \nu) \cdot \mathbf{v}^\top \cdot \hat{\delta} \cdot \hat{\Lambda} \cdot \mathbf{m}] \right] - \left[ \mathcal{E}_n[\bar{\mathbf{e}}^{-1} \cdot \hat{\Lambda} \cdot \mathbf{m}] \right] \right) ==$$

$$\boxed{\text{TAB}} \text{Det}[\mathbf{m}] \left( \left[ \mathcal{E}_{d-n}[\bar{\mathbf{m}}^{-1} \cdot \hat{\Lambda} \cdot \mathbf{e} + (\mathbf{N} \bar{\mathbf{e}}^{-1} \cdot \mathbf{v} + \mathbf{M} \bar{\mathbf{m}}^{-1} \cdot \mathbf{v} + \mu - \nu) \cdot \mathbf{v}^\top \cdot \hat{\delta} \cdot \hat{\Lambda} \cdot \mathbf{e}] \right] - \left[ \mathcal{E}_{d-n}[\bar{\mathbf{m}}^{-1} \cdot \hat{\Lambda} \cdot \mathbf{e}] \right] \right) // \blacksquare \mathbf{n}$$

True True True True True True

$$\text{In[106]} := \mathbf{N} \text{Det}[\mathbf{e}] \left[ \mathcal{E}_n[\bar{\mathbf{e}}^{-1} \cdot \bar{\hat{\Lambda}}^{-1} \cdot \mathbf{m}] \right] + \mathbf{M} \text{Det}[\mathbf{m}] \left[ \mathcal{E}_{d-n}[\bar{\mathbf{m}}^{-1} \cdot \bar{\hat{\Lambda}}^{-1} \cdot \mathbf{e}] \right] +$$

$$\boxed{\text{RET}} + \text{Det}[\mathbf{e}] \left( \left[ \mathcal{E}_n[\bar{\mathbf{e}}^{-1} \cdot \hat{\Lambda} \cdot \mathbf{m} + (\mathbf{N} \bar{\mathbf{e}}^{-1} \cdot \mathbf{v} + \mathbf{M} \bar{\mathbf{m}}^{-1} \cdot \mathbf{v}) \cdot \mathbf{v}^\top \cdot \hat{\delta} \cdot \hat{\Lambda} \cdot \mathbf{m}] \right] - \right.$$

$$\left. \left[ \mathcal{E}_n[\bar{\mathbf{e}}^{-1} \cdot \hat{\Lambda} \cdot \mathbf{m} - (\mu - \nu) \cdot \mathbf{v}^\top \cdot \hat{\delta} \cdot \hat{\Lambda} \cdot \mathbf{m}] \right] \right) // \blacksquare \text{\$NdEn}$$

True True True True True True

$$\text{In[107]} := \mathbf{N} \text{Det}[\mathbf{e}] \left[ \mathcal{E}_n[\bar{\mathbf{e}}^{-1} \cdot \bar{\hat{\Lambda}}^{-1} \cdot \mathbf{m}] \right] + \mathbf{M} \text{Det}[\mathbf{m}] \left[ \mathcal{E}_{d-n}[\bar{\mathbf{m}}^{-1} \cdot \bar{\hat{\Lambda}}^{-1} \cdot \mathbf{e}] \right] +$$

$$\boxed{\text{RET}} + \text{Det}[\mathbf{m}] \left( \left[ \mathcal{E}_{d-n}[\bar{\mathbf{m}}^{-1} \cdot \hat{\Lambda} \cdot \mathbf{e} + (\mathbf{N} \bar{\mathbf{e}}^{-1} \cdot \mathbf{v} + \mathbf{M} \bar{\mathbf{m}}^{-1} \cdot \mathbf{v}) \cdot \mathbf{v}^\top \cdot \hat{\delta} \cdot \hat{\Lambda} \cdot \mathbf{e}] \right] - \right.$$

$$\left. \left[ \mathcal{E}_{d-n}[\bar{\mathbf{m}}^{-1} \cdot \hat{\Lambda} \cdot \mathbf{e} - (\mu - \nu) \cdot \mathbf{v}^\top \cdot \hat{\delta} \cdot \hat{\Lambda} \cdot \mathbf{e}] \right] \right) // \blacksquare \text{\$NdEn}$$

True True True True True True

True True True True True True

True True True True True True

## **$N_{\det}(e) \leq e_n(S)$ Derivation track 4**

True True True True True True

|      |      |      |      |      |      |
|------|------|------|------|------|------|
| True | True | True | True | True | True |
|------|------|------|------|------|------|

True True True True True True

True True True True True True

True True True True True True



$$\text{In[121]}:= \mathbf{NDet}[\mathbf{e}] \left( \boxed{\mathcal{E}_n[\mathbf{m} \cdot \hat{\mathbf{e}}^1]} + \boxed{\text{RET}} + \sum_{k=1}^n (-1)^{k-1} \boxed{\mathcal{E}_{n-k}[\mathbf{m} \cdot \hat{\mathbf{e}}^1]} \mathbf{p}^\top \cdot \hat{\boldsymbol{\delta}} \cdot \left( \mathbf{m} \cdot \hat{\mathbf{e}}^1 \right) \cdot \mathbf{e} \cdot \left( \frac{1}{\lambda+1} \hat{\mathbf{e}}^1 \cdot \mathbf{p} - \mathbf{N}^{-1} \mathbf{v} \right) \right) +$$

$$\boxed{\text{RET}} + \mathbf{MDet}[\mathbf{m}] \left( \boxed{\mathcal{E}_{d-n}[\mathbf{e} \cdot \hat{\mathbf{m}}^1]} + \boxed{\text{RET}} + \sum_{k=1}^{d-n} (-1)^{k-1} \boxed{\mathcal{E}_{d-n-k}[\mathbf{e} \cdot \hat{\mathbf{m}}^1]} \mathbf{p}^\top \cdot \hat{\boldsymbol{\delta}} \cdot \left( \mathbf{e} \cdot \hat{\mathbf{m}}^1 \right) \cdot \mathbf{m} \cdot \left( \frac{1}{\lambda+1} \hat{\mathbf{m}}^1 \cdot \mathbf{p} + \mathbf{M}^{-1} \boldsymbol{\mu} \right) \right) // \blacksquare \text{\$NdEn}$$

True True True True True True

$$\text{In[122]}:= \mathbf{NDet}[\mathbf{e}] \boxed{\mathcal{E}_n[\mathbf{m} \cdot \hat{\mathbf{e}}^1 \cdot \left( \hat{\mathbf{I}} + \left( \frac{1}{\lambda+1} \mathbf{p} - \mathbf{N}^{-1} \mathbf{e} \cdot \mathbf{v} \right) \cdot \mathbf{p}^\top \cdot \hat{\boldsymbol{\delta}} \right)]} +$$

$$\boxed{\text{RET}} + \mathbf{MDet}[\mathbf{m}] \boxed{\mathcal{E}_{d-n}[\mathbf{e} \cdot \hat{\mathbf{m}}^1 \cdot \left( \hat{\mathbf{I}} + \left( \frac{1}{\lambda+1} \mathbf{p} + \mathbf{M}^{-1} \mathbf{m} \cdot \boldsymbol{\mu} \right) \cdot \mathbf{p}^\top \cdot \hat{\boldsymbol{\delta}} \right)]} // \blacksquare \text{\$NdEn}$$

True True True True True True

$$\text{In[123]}:= \mathbf{NDet}[\mathbf{e}] \boxed{\mathcal{E}_n[\mathbf{m} \cdot \hat{\mathbf{e}}^1 \cdot (\hat{\boldsymbol{\Lambda}} - \mathbf{N}^{-1} \mathbf{e} \cdot \mathbf{v} \cdot \mathbf{p}^\top \cdot \hat{\boldsymbol{\delta}})]} +$$

$$\boxed{\text{RET}} + \mathbf{MDet}[\mathbf{m}] \boxed{\mathcal{E}_{d-n}[\mathbf{e} \cdot \hat{\mathbf{m}}^1 \cdot (\hat{\boldsymbol{\Lambda}} + \mathbf{M}^{-1} \mathbf{m} \cdot \boldsymbol{\mu} \cdot \mathbf{p}^\top \cdot \hat{\boldsymbol{\delta}})]} // \blacksquare \text{\$NdEn}$$

True True True True True True

$$\text{In[124]}:= \mathbf{NDet}[\mathbf{e}] \boxed{\mathcal{E}_n[\mathbf{m} \cdot \hat{\mathbf{e}}^1 \cdot \hat{\boldsymbol{\Lambda}} - \mathbf{N}^{-1} \mathbf{m} \cdot \mathbf{v} \cdot \mathbf{p}^\top \cdot \hat{\boldsymbol{\delta}}]} +$$

$$\boxed{\text{RET}} + \mathbf{MDet}[\mathbf{m}] \boxed{\mathcal{E}_{d-n}[\mathbf{e} \cdot \hat{\mathbf{m}}^1 \cdot \hat{\boldsymbol{\Lambda}} + \mathbf{M}^{-1} \mathbf{e} \cdot \boldsymbol{\mu} \cdot \mathbf{p}^\top \cdot \hat{\boldsymbol{\delta}}]} // \blacksquare \text{\$NdEn}$$

True True True True True True

$$\text{In[125]}:= \mathbf{NDet}[\mathbf{e}] \boxed{\mathcal{E}_n[\hat{\mathbf{e}}^1 \cdot \hat{\boldsymbol{\Lambda}} \cdot \mathbf{m} - \mathbf{N}^{-1} \mathbf{v} \cdot \mathbf{v}^\top \cdot \hat{\boldsymbol{\delta}} \cdot \hat{\boldsymbol{\Lambda}} \cdot \mathbf{m}]} +$$

$$\boxed{\text{RET}} + \mathbf{MDet}[\mathbf{m}] \boxed{\mathcal{E}_{d-n}[\hat{\mathbf{m}}^1 \cdot \hat{\boldsymbol{\Lambda}} \cdot \mathbf{e} + \mathbf{M}^{-1} \boldsymbol{\mu} \cdot \mathbf{v}^\top \cdot \hat{\boldsymbol{\delta}} \cdot \hat{\boldsymbol{\Lambda}} \cdot \mathbf{e}]} // \blacksquare \text{\$NdEn}$$

True True True True True True

$$\text{In[126]}:= \mathbf{NDet}[\mathbf{e}] \boxed{\mathcal{E}_n[\left( \hat{\mathbf{e}}^1 - \mathbf{N}^{-1} \mathbf{v} \cdot \mathbf{v}^\top \cdot \hat{\boldsymbol{\delta}} \right) \cdot \hat{\boldsymbol{\Lambda}} \cdot \mathbf{m}]} +$$

$$\boxed{\text{RET}} + \mathbf{MDet}[\mathbf{m}] \boxed{\mathcal{E}_{d-n}[\left( \hat{\mathbf{m}}^1 + \mathbf{M}^{-1} \boldsymbol{\mu} \cdot \mathbf{v}^\top \cdot \hat{\boldsymbol{\delta}} \right) \cdot \hat{\boldsymbol{\Lambda}} \cdot \mathbf{e}]} // \blacksquare \text{\$NdEn}$$

True True True True True True

$$\text{In[127]}:= \mathbf{NDet}[\mathbf{e}] \boxed{\mathcal{E}_n[\left( \hat{\mathbf{e}}^1 + \mathbf{N}^{-1} \left( \frac{\lambda}{\lambda+1} \mathbf{N} \hat{\mathbf{e}}^1 \cdot \mathbf{v} - \mathbf{v} \right) \cdot \mathbf{v}^\top \cdot \hat{\boldsymbol{\delta}} \cdot \hat{\boldsymbol{\Lambda}} \right) \cdot \mathbf{m}]} +$$

$$\boxed{\text{RET}} + \mathbf{MDet}[\mathbf{m}] \boxed{\mathcal{E}_{d-n}[\left( \hat{\mathbf{m}}^1 + \mathbf{M}^{-1} \left( \frac{\lambda}{\lambda+1} \mathbf{M} \hat{\mathbf{m}}^1 \cdot \mathbf{v} + \boldsymbol{\mu} \right) \cdot \mathbf{v}^\top \cdot \hat{\boldsymbol{\delta}} \cdot \hat{\boldsymbol{\Lambda}} \right) \cdot \mathbf{e}]} // \blacksquare \text{\$NdEn}$$

True True True True True True

### **$Ne_n(S)$ Derivation track 7 (used to get EoM)**

Now the equations contain  $p$ 's outside the elementary symmetric polynomials (the parts which depend on  $p$  are highlighted in yellow). These equations are nice to be varied w.r.t.  $p$ .

$$\begin{aligned} \text{In[128]} := & \mathbf{N} \text{Det}[\mathbf{e}] \left( \boxed{\mathcal{E}_n[\mathbf{m} \cdot \bar{\mathbf{e}}^{-1}]} + \boxed{\text{RET}} + \sum_{k=1}^n (-1)^{k-1} \boxed{\mathcal{E}_{n-k}[\mathbf{m} \cdot \bar{\mathbf{e}}^{-1}]} \mathbf{p}^1 \cdot \hat{\delta} \cdot \left( \mathbf{m} \cdot \bar{\mathbf{e}}^{-1} \right) \cdot \mathbf{e} \cdot \left( \frac{1}{\lambda+1} \bar{\mathbf{e}}^{-1} \cdot \mathbf{p} - \mathbf{N}^{-1} \mathbf{v} \right) \right) + \\ & \boxed{\text{RET}} + \mathbf{M} \text{Det}[\mathbf{m}] \left( \boxed{\mathcal{E}_{d-n}[\mathbf{e} \cdot \bar{\mathbf{m}}^{-1}]} + \boxed{\text{RET}} + \right. \\ & \left. \sum_{k=1}^{d-n} (-1)^{k-1} \boxed{\mathcal{E}_{d-n-k}[\mathbf{e} \cdot \bar{\mathbf{m}}^{-1}]} \mathbf{p}^1 \cdot \hat{\delta} \cdot \left( \mathbf{e} \cdot \bar{\mathbf{m}}^{-1} \right) \cdot \mathbf{m} \cdot \left( \frac{1}{\lambda+1} \bar{\mathbf{m}}^{-1} \cdot \mathbf{p} + \mathbf{M}^{-1} \mu \right) \right) // \blacksquare \$\text{NdEn} \end{aligned}$$

True True True True True True

$$\begin{aligned} \text{In[129]} := & \mathbf{N} \text{Det}[\mathbf{e}] \boxed{\mathcal{E}_n[\mathbf{m} \cdot \bar{\mathbf{e}}^{-1}]} + \boxed{\text{RET}} + \text{Det}[\mathbf{e}] \sum_{k=1}^n (-1)^{k-1} \boxed{\mathcal{E}_{n-k}[\mathbf{m} \cdot \bar{\mathbf{e}}^{-1}]} \mathbf{p}^1 \cdot \hat{\delta} \cdot \left( \mathbf{m} \cdot \bar{\mathbf{e}}^{-1} \right) \cdot \mathbf{e} \cdot \left( \frac{1}{\lambda+1} \mathbf{N} \bar{\mathbf{e}}^{-1} \cdot \mathbf{p} - \mathbf{v} \right) + \\ & \boxed{\text{RET}} + \mathbf{M} \text{Det}[\mathbf{m}] \boxed{\mathcal{E}_{d-n}[\mathbf{e} \cdot \bar{\mathbf{m}}^{-1}]} + \boxed{\text{RET}} + \\ & \text{Det}[\mathbf{m}] \sum_{k=1}^{d-n} (-1)^{k-1} \boxed{\mathcal{E}_{d-n-k}[\mathbf{e} \cdot \bar{\mathbf{m}}^{-1}]} \mathbf{p}^1 \cdot \hat{\delta} \cdot \left( \mathbf{e} \cdot \bar{\mathbf{m}}^{-1} \right) \cdot \mathbf{m} \cdot \left( \frac{1}{\lambda+1} \mathbf{M} \bar{\mathbf{m}}^{-1} \cdot \mathbf{p} + \mu \right) // \blacksquare \$\text{NdEn} \end{aligned}$$

True True True True True True

$$\begin{aligned} \text{In[130]} := & \left( \mathbf{N} \text{Det}[\mathbf{e}] \boxed{\mathcal{E}_n[\mathbf{m} \cdot \bar{\mathbf{e}}^{-1}]} + \boxed{\text{RET}} + \right. \\ & \left. \text{Det}[\mathbf{e}] \sum_{k=1}^n (-1)^{k-1} \boxed{\mathcal{E}_{n-k}[\mathbf{m} \cdot \bar{\mathbf{e}}^{-1}]} \mathbf{p}^1 \cdot \hat{\delta} \cdot \left( \mathbf{m} \cdot \bar{\mathbf{e}}^{-1} \right) \cdot \mathbf{e} \cdot \left( \frac{1}{\lambda+1} \mathbf{N} \bar{\mathbf{e}}^{-1} \cdot \mathbf{p} - \mathbf{v} \right) \right) + \\ & \boxed{\text{RET}} + \left( \mathbf{M} \text{Det}[\mathbf{e}] \boxed{\mathcal{E}_{n-1}[\mathbf{m} \cdot \bar{\mathbf{e}}^{-1}]} + \boxed{\text{RET}} + \text{Det}[\mathbf{e}] \right. \\ & \left. \sum_{k=1}^n (-1)^{k-1} \boxed{\mathcal{E}_{n-k}[\mathbf{m} \cdot \bar{\mathbf{e}}^{-1}]} \mathbf{p}^1 \cdot \hat{\delta} \cdot \left( \mathbf{m} \cdot \bar{\mathbf{e}}^{-1} \right) \cdot \mathbf{e} \cdot \left( \frac{1}{\lambda+1} \mathbf{M} \bar{\mathbf{m}}^{-1} \cdot \mathbf{p} + \mu \right) \right) // \blacksquare \$\text{NdEn} \end{aligned}$$

True True True True True True

$$\begin{aligned} \text{In[131]} := & \left( \mathbf{N} \text{Det}[\mathbf{e}] \boxed{\mathcal{E}_n[\mathbf{m} \cdot \bar{\mathbf{e}}^{-1}]} + \boxed{\text{RET}} + \right. \\ & \left. \text{Det}[\mathbf{e}] \sum_{k=1}^n (-1)^{k-1} \boxed{\mathcal{E}_{n-k}[\mathbf{m} \cdot \bar{\mathbf{e}}^{-1}]} \mathbf{p}^1 \cdot \hat{\delta} \cdot \left( \mathbf{m} \cdot \bar{\mathbf{e}}^{-1} \right) \cdot \mathbf{e} \cdot \left( \frac{1}{\lambda+1} \mathbf{N} \bar{\mathbf{e}}^{-1} \cdot \mathbf{p} - \mathbf{v} \right) \right) + \\ & \boxed{\text{RET}} + \left( \mathbf{M} \text{Det}[\mathbf{m}] \boxed{\mathcal{E}_{d-n}[\mathbf{e} \cdot \bar{\mathbf{m}}^{-1}]} + \boxed{\text{RET}} + \text{Det}[\mathbf{e}] \right. \\ & \left. \sum_{k=1}^n (-1)^{k-1} \boxed{\mathcal{E}_{n-k}[\mathbf{m} \cdot \bar{\mathbf{e}}^{-1}]} \mathbf{p}^1 \cdot \hat{\delta} \cdot \left( \mathbf{m} \cdot \bar{\mathbf{e}}^{-1} \right) \cdot \mathbf{e} \cdot \left( \frac{1}{\lambda+1} \mathbf{M} \bar{\mathbf{m}}^{-1} \cdot \mathbf{p} + \mu \right) \right) // \blacksquare \$\text{NdEn} \end{aligned}$$

True True True True True True

Finally, we have  $\boxed{Ne_n(S)}$  which is **suitable to be varied**

$$\begin{aligned} \text{In[132]} := & \mathbf{N} \boxed{\mathcal{E}_n[\mathbf{m} \cdot \bar{\mathbf{e}}^{-1}]} + \mathbf{M} \boxed{\mathcal{E}_{n-1}[\mathbf{m} \cdot \bar{\mathbf{e}}^{-1}]} + \\ & \boxed{\text{RET}} + \sum_{k=1}^n (-1)^{k-1} \boxed{\mathcal{E}_{n-k}[\mathbf{m} \cdot \bar{\mathbf{e}}^{-1}]} \mathbf{p}^1 \cdot \hat{\delta} \cdot \left( \mathbf{m} \cdot \bar{\mathbf{e}}^{-1} \right) \cdot \mathbf{e} \cdot \left( \frac{1}{\lambda+1} \mathbf{N} \bar{\mathbf{e}}^{-1} \cdot \mathbf{p} + \frac{1}{\lambda+1} \mathbf{M} \bar{\mathbf{m}}^{-1} \cdot \mathbf{p} + \mu - \mathbf{v} \right) // \blacksquare \$\text{NEEn} \end{aligned}$$

True True True True True True

$$\text{In[133]} := \mathbf{N} \left[ \mathcal{E}_n \left[ \mathbf{m} \cdot \hat{\mathbf{e}}^{-1} \right] \right] + \mathbf{M} \left[ \mathcal{E}_{n-1} \left[ \mathbf{m} \cdot \hat{\mathbf{e}}^{-1} \right] \right] +$$

$$\left[ \text{RET} \right] + \sum_{k=1}^n (-1)^{k-1} \left[ \mathcal{E}_{n-k} \left[ \mathbf{m} \cdot \hat{\mathbf{e}}^{-1} \right] \right] \mathbf{p}^\top \cdot \hat{\delta} \cdot \left( \mathbf{m} \cdot \hat{\mathbf{e}}^{-1} \right) \cdot \mathbf{m} \cdot \left( \left( \mathbf{N} \hat{\mathbf{e}}^{-1} + \mathbf{M} \hat{\mathbf{m}}^{-1} \right) \cdot \left( \frac{1}{\lambda+1} \mathbf{p} \right) + \mu - \nu \right) // \blacksquare \$N \mathbf{E} n$$

True True True True True True

The equations of motion will be obtained from the following:

$$\text{In[134]} := \mathbf{N} \left[ \mathcal{E}_n \left[ \mathbf{m} \cdot \hat{\mathbf{e}}^{-1} \right] \right] + \mathbf{M} \left[ \mathcal{E}_{n-1} \left[ \mathbf{m} \cdot \hat{\mathbf{e}}^{-1} \right] \right] +$$

$$\left[ \text{RET} \right] + \sum_{k=1}^n (-1)^{k-1} \left[ \mathcal{E}_{n-k} \left[ \mathbf{m} \cdot \hat{\mathbf{e}}^{-1} \right] \right] \mathbf{p}^\top \cdot \hat{\delta} \cdot \left( \mathbf{m} \cdot \hat{\mathbf{e}}^{-1} \right) \cdot \mathbf{m} \cdot \left( \left( \mathbf{N} \hat{\mathbf{e}}^{-1} + \mathbf{M} \hat{\mathbf{m}}^{-1} \right) \cdot \left( \frac{1}{\lambda+1} \mathbf{p} \right) + \mu - \nu \right) // \blacksquare \$N \mathbf{E} n$$

True True True True True True

## Part 3

### Equations of Motion for $p$

The starting point is  $Ne_n(S)$

`In[135] := random$g[]; If[Not@ValueQ[g], Text["Established "]] N  $\mathcal{E}_n[S]$  Text[":"] //  $\blacksquare$`

$$\text{In[136]} := \mathbf{N} \left[ \mathcal{E}_n \left[ \mathbf{m} \cdot \hat{\mathbf{e}}^{-1} \right] \right] + \mathbf{M} \left[ \mathcal{E}_{n-1} \left[ \mathbf{m} \cdot \hat{\mathbf{e}}^{-1} \right] \right] +$$

$$\left[ \text{RET} \right] + \sum_{k=1}^n (-1)^{k-1} \left[ \mathcal{E}_{n-k} \left[ \mathbf{m} \cdot \hat{\mathbf{e}}^{-1} \right] \right] \mathbf{p}^\top \cdot \hat{\delta} \cdot \left( \mathbf{m} \cdot \hat{\mathbf{e}}^{-1} \right) \cdot \mathbf{m} \cdot \left( \left( \mathbf{N} \hat{\mathbf{e}}^{-1} + \mathbf{M} \hat{\mathbf{m}}^{-1} \right) \cdot \left( \frac{1}{\lambda+1} \mathbf{p} \right) + \mu - \nu \right) // \blacksquare \$N \mathbf{E} n$$

True True True True True True

$$\text{In[137]} := \mathbf{N} \left[ \mathcal{E}_n \left[ \mathbf{m} \cdot \hat{\mathbf{e}}^{-1} \right] \right] + \mathbf{M} \left[ \mathcal{E}_{n-1} \left[ \mathbf{m} \cdot \hat{\mathbf{e}}^{-1} \right] \right] +$$

$$\left[ \text{RET} \right] + \mathbf{p}^\top \cdot \left[ \hat{\delta} \cdot \mathbf{y}_{n-1} \left[ \mathbf{m} \cdot \hat{\mathbf{e}}^{-1} \right] \right] \cdot \mathbf{m} \cdot \left( \left( \mathbf{N} \hat{\mathbf{e}}^{-1} + \mathbf{M} \hat{\mathbf{m}}^{-1} \right) \cdot \left( \frac{1}{\lambda+1} \mathbf{p} \right) + \mu - \nu \right) // \blacksquare \$N \mathbf{E} n$$

True True True True True True

$$\text{In[138]} := \mathbf{N} \left[ \mathcal{E}_n \left[ \mathbf{m} \cdot \hat{\mathbf{e}}^{-1} \right] \right] + \mathbf{M} \left[ \mathcal{E}_{n-1} \left[ \mathbf{m} \cdot \hat{\mathbf{e}}^{-1} \right] \right] +$$

$$\left[ \text{RET} \right] + \mathbf{v}^\top \cdot \hat{\Lambda}^\top \cdot \left[ \hat{\delta} \cdot \mathbf{y}_{n-1} \left[ \mathbf{m} \cdot \hat{\mathbf{e}}^{-1} \right] \right] \cdot \mathbf{m} \cdot \left( \frac{\lambda}{\lambda+1} \left( \mathbf{N} \hat{\mathbf{e}}^{-1} + \mathbf{M} \hat{\mathbf{m}}^{-1} \right) \cdot \mathbf{v} + \mu - \nu \right) // \blacksquare \$N \mathbf{E} n$$

True True True True True True

The variation of  $Ne_n(S)$  with respect to  $p = \lambda v$

The variation  $\partial \mathcal{V} / \partial p$  is established using the following two identities:

$$\partial \left( \mathbf{p}^\top \cdot \diamond \right) / \partial \mathbf{p} = \diamond^\top,$$

$$\partial \left( \diamond \cdot \frac{\mathbf{p}}{\lambda+1} \right) / \partial \mathbf{p} = \frac{1}{\lambda+1} \diamond \cdot \hat{\Lambda}^{-1} \text{ where } \hat{\Lambda}^{-1} = \hat{\Gamma} - \frac{1}{\lambda(\lambda+1)} \mathbf{p} \mathbf{p}^\top \hat{\delta},$$

where  $\diamond$  and  $\blacklozenge$  are assumed not to depend on  $p$ .



```
In[139]:= If[ValueQ[g],
  δ$V[n_] := (δ · yn-1[m · e-1] · m · (1/(λ+1) (N e-1 + M m-1) · p + μ - ν))τ +
  (pτ · δ · yn-1[m · e-1] · m · (1/(λ+1) (N e-1 + M m-1) · λ̂))τ,
  Text["Established "] δ$V[n] Text[":"] // ■
]
```

```
In[140]:= δ$V[n]τ == (δ · yn-1[m · e-1] · m · (λ/(λ+1) (N e-1 + M m-1) · v + μ - ν) +
  RET + 1/(λ+1) (vτ · λ̂τ · δ · yn-1[m · e-1] · m · (N e-1 + M m-1) · λ̂-1)τ // ■n
```

True True True True True True

```
In[141]:= δ$V[n]τ == (δ · yn-1[m · e-1] · m · (N e-1 + M m-1) · v + μ - ν) +
  RET + 1/(λ+1) (λ̂τ · δ · yn-1[m · e-1] · m · (N e-1 + M m-1) · λ̂-1)τ · v +
  RET - 1/(λ+1) (δ · yn-1[m · e-1] · m · (N e-1 + M m-1) · v) // ■n
```

True True True True True True

If  $\hat{\delta} \hat{\Lambda} m e^{-1}$  is symmetric, then the following holds:

```
In[142]:= symmetrize$gE[]; δ · λ̂ · m · e-1 == (δ · λ̂ · m · e-1)τ // ■n
```

True True True True True True  
True True True True True True

```
In[143]:= Inverse[λ̂] · f̂ == e-1 · λ̂ · m · e-1 · λ̂-1 · m // ■
```

True

```
In[144]:= δ · λ̂ · (m · e-1)n == (δ · λ̂ · (m · e-1)n)τ // ■n
```

True True True True True True

This means that  $\hat{\delta} \hat{\Lambda} f(m e^{-1})$  is symmetric for any analytic function  $f$ .

```
In[145]:= δ · λ̂ · MatrixFunction[Log, m · e-1] == (δ · λ̂ · MatrixFunction[Log, m · e-1])τ // ■
```

True

Moreover, we have the following identities that involve  $Y_n$ .

```
In[146]:= λ̂τ · δ · yn-1[m · e-1] == (λ̂τ · δ · yn-1[m · e-1])τ // ■n
```

True True True True True True

```
In[147]:= vτ · λ̂τ · δ · yn-1[m · e-1] · λ̂-1 == vτ · (λ̂τ · δ · yn-1[m · e-1])τ · λ̂-1 // ■n
```

True True True True True True

$$\text{In[148]:= } \mathbf{v}^\top \cdot \hat{\Lambda}^\top \cdot \hat{\delta} \cdot \mathbf{y}_{n-1} [\mathbf{m} \cdot \hat{\mathbf{e}}^{-1}] \cdot \hat{\Lambda}^{-1} == \left( \hat{\Lambda}^\top \cdot \hat{\delta} \cdot \mathbf{y}_{n-1} [\mathbf{m} \cdot \hat{\mathbf{e}}^{-1}] \cdot \mathbf{v} \right)^\top \cdot \hat{\Lambda}^{-1} // \text{■n}$$

True True True True True True

$$\text{In[149]:= } \mathbf{v}^\top \cdot \hat{\Lambda}^\top \cdot \hat{\delta} \cdot \mathbf{y}_{n-1} [\mathbf{m} \cdot \hat{\mathbf{e}}^{-1}] \cdot \hat{\Lambda}^{-1} == \left( \hat{\delta} \cdot \mathbf{y}_{n-1} [\mathbf{m} \cdot \hat{\mathbf{e}}^{-1}] \cdot \mathbf{v} \right)^\top // \text{■n}$$

True True True True True True

*contd. For the symmetric  $\hat{\delta} \hat{\Lambda} m e^{-1}$ , we have:*

$$\text{In[150]:= } \delta \mathcal{S} \mathbf{V} [\mathbf{n}]^\top == \left( \hat{\delta} \cdot \mathbf{y}_{n-1} [\mathbf{m} \cdot \hat{\mathbf{e}}^{-1}] \cdot \mathbf{m} \cdot \left( \frac{\lambda}{\lambda + 1} \left( \mathbf{N} \hat{\mathbf{e}}^{-1} + \mathbf{M} \hat{\mathbf{m}}^{-1} \right) \cdot \mathbf{v} + \mu - \mathbf{v} \right) + \right. \\ \left. \text{RET} + \frac{1}{\lambda + 1} \left( \mathbf{v}^\top \cdot \hat{\Lambda}^\top \cdot \hat{\delta} \cdot \mathbf{y}_{n-1} [\mathbf{m} \cdot \hat{\mathbf{e}}^{-1}] \cdot \mathbf{m} \cdot \left( \mathbf{N} \hat{\mathbf{e}}^{-1} + \mathbf{M} \hat{\mathbf{m}}^{-1} \right) \cdot \hat{\Lambda}^{-1} \right)^\top \right) // \text{■n}$$

True True True True True True

$$\text{In[151]:= } \delta \mathcal{S} \mathbf{V} [\mathbf{n}]^\top == \left( \hat{\delta} \cdot \mathbf{y}_{n-1} [\mathbf{m} \cdot \hat{\mathbf{e}}^{-1}] \cdot \mathbf{m} \cdot \left( \frac{\lambda}{\lambda + 1} \left( \mathbf{N} \hat{\mathbf{e}}^{-1} + \mathbf{M} \hat{\mathbf{m}}^{-1} \right) \cdot \mathbf{v} + \mu - \mathbf{v} \right) + \right. \\ \left. \text{RET} + \frac{1}{\lambda + 1} \left( \hat{\delta} \cdot \mathbf{y}_{n-1} [\mathbf{m} \cdot \hat{\mathbf{e}}^{-1}] \cdot \mathbf{m} \cdot \left( \mathbf{N} \hat{\mathbf{e}}^{-1} + \mathbf{M} \hat{\mathbf{m}}^{-1} \right) \cdot \mathbf{v} \right) \right) // \text{■n}$$

True True True True True True

$$\text{In[152]:= } \delta \mathcal{S} \mathbf{V} [\mathbf{n}]^\top == \hat{\delta} \cdot \mathbf{y}_{n-1} [\mathbf{m} \cdot \hat{\mathbf{e}}^{-1}] \cdot \mathbf{m} \cdot \left( \left( \mathbf{N} \hat{\mathbf{e}}^{-1} + \mathbf{M} \hat{\mathbf{m}}^{-1} \right) \cdot \mathbf{v} + \mu - \mathbf{v} \right) // \text{■n}$$

True True True True True True

$$\text{In[153]:= } \delta \mathcal{S} \mathbf{V} [\mathbf{n}]^\top == \hat{\delta} \cdot \mathbf{y}_{n-1} [\mathbf{m} \cdot \hat{\mathbf{e}}^{-1}] \cdot \mathbf{m} \cdot \Delta \mathbf{n} // \text{■n}$$

True True True True True True

## Conclusion: $\Delta n = 0$

The EoM for  $p = \lambda \mathbf{v}$  yields the shift redefinition together with the spatial vielbein symmetrization (which is equivalent to the principal square root):

$$\mathbf{v} = \mathbf{N} \mathbf{e}^{-1} \mathbf{v} + \mathbf{M} \mathbf{m}^{-1} \mathbf{v} + \mu$$

$$\hat{\delta} \hat{\Lambda} m e^{-1} = \left( \hat{\delta} \hat{\Lambda} m e^{-1} \right)^\top$$

In[154]:= **finalizeProofs[]**

Memory used: 29.332 + 1.514 MBy

Session time: 4.068 + 7.878 s

CPU time: 0.344 + 4.023 s
